# Supplementary material for: Pushing the limits of optical information storage using deep learning
Source: arXiv:1805.03468 ancillary file (2018-10-09)
Supplement: Supplementary file 1 [file wiecha_supinfo.pdf]

# Supporting Informations to: Pushing the limits of optical information storage using deep learning

Peter R. Wiecha,[1,*] Aurélie Lecestre,[2] Nicolas Mallet,[2] and Guilhem Larrieu[2]

[1] *CEMES, Université de Toulouse, CNRS, Toulouse, France*

[2] *LAAS, Université de Toulouse, CNRS, INP, Toulouse, France*

## I. SCANNING ELECTRON MICROSCOPY IMAGES

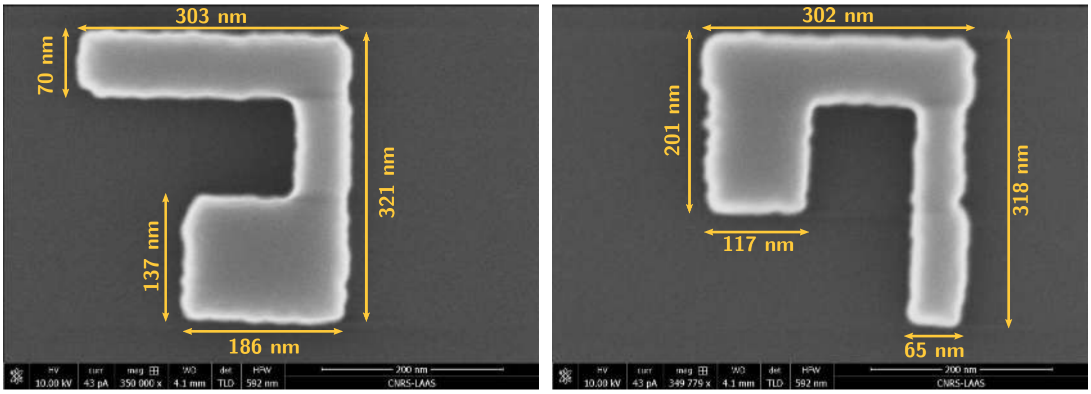


FIG. S.1. **SEM images of "0100" and "0010" 4 bit structures** Scanning electron microscopy (SEM) images of the mirrored 4 bit structures "0100" and "0010". The fabrication clearly induces orientational-dependent differences between $X$- and $Y$-aligned structural features, hence the non-symmetric spectral response for $X$ and $Y$ polarization.

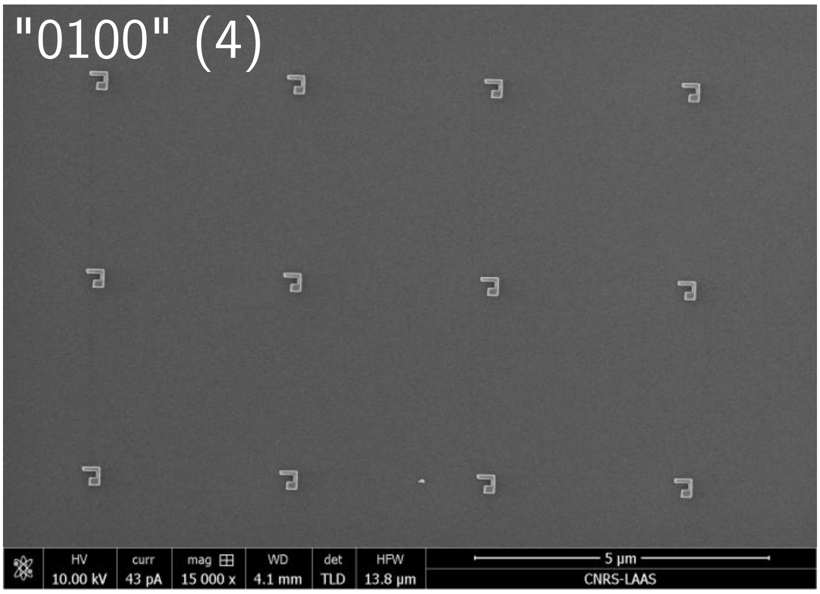


FIG. S.2. **SEM images of several copies of "0100" 4 bit geometry** SEM image of an array of 12 copies of the 4-bit nanostructure "0100" (decimal "4"). Fabrication-induced structural variations as well as small defects (e.g. small particle close to bottom row, second right) cause variations in the scattering spectra from individual copies.

---

* e-mail : peter.wiecha@cemes.fr

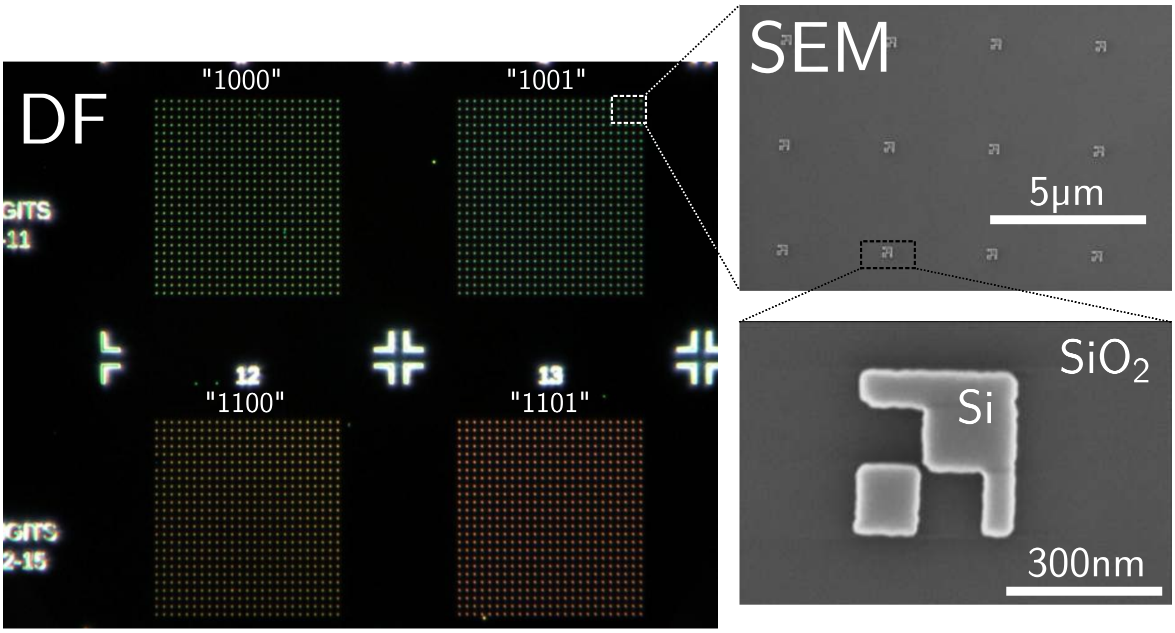


FIG. S.3. **Darkfield microscopy and SEM images of selected 4 bit structures** $X$-polarization filtered DF microscopy (left) and SEM images (right) of copies of the 4-bit nanostructure “1001”, decimal “9”).

## II. MEASURED SPECTRA FOR ALL DATASETS

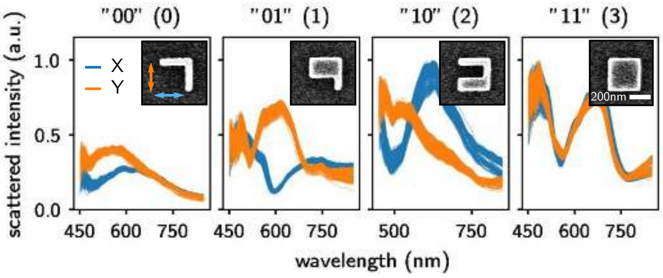


FIG. S.4. **Acquired spectra for 2 bit experimental datasets** Superposition of all acquired spectra (625 copies per structure). $X$ polarization is shown with blue lines, $Y$ polarization with orange lines. Insets show representative SEM images of the structure corresponding to the respective bit sequences. SEM images are $600 \times 600\,\mathrm{nm}^2$ large, scalebar in “11” is 100 nm.

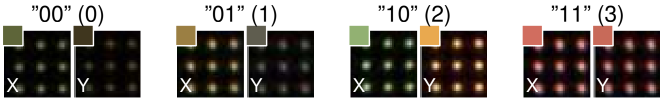


FIG. S.5. **DF microscopy image RGB color for 2 bit structures** RGB color from polarized DF microscopy images for 9 selected copies of each structure and polarization case (left subplots: $X$, right subplots: $Y$ polarization). The color-box insets at the top right corresponds to the average RGB color of the shown structures.

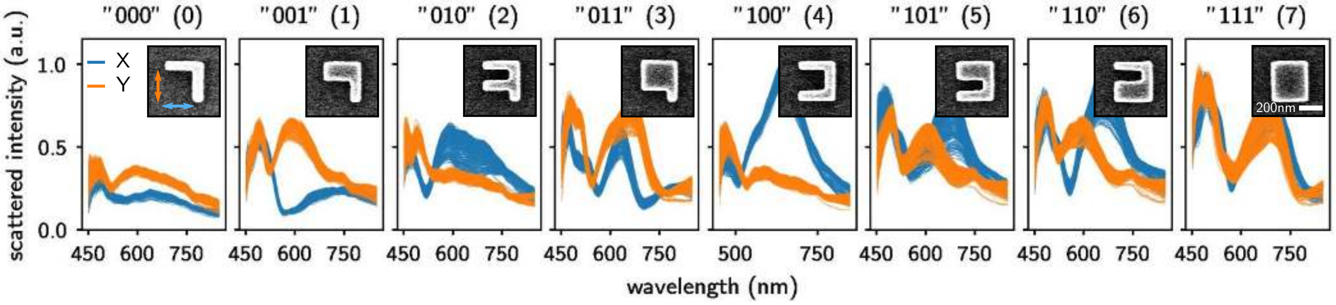


FIG. S.6. **Acquired spectra for 3 bit experimental datasets** Same as figure S.4 but for the 3 bit dataset.

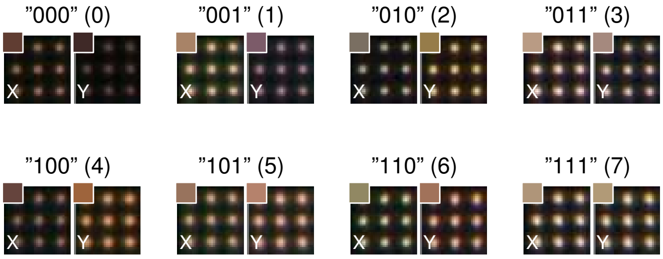


FIG. S.7. **DF microscopy image RGB color for 3 bit structures** Same as figure S.5, but for the 3 bit structures. Slightly different RGB colors for similar structures between the datasets (2 bit “11”, 3 bit “111”) are a result of different white-balance of the CDD camera. We note that white-balance was always constant during the acquisition of each entire set.

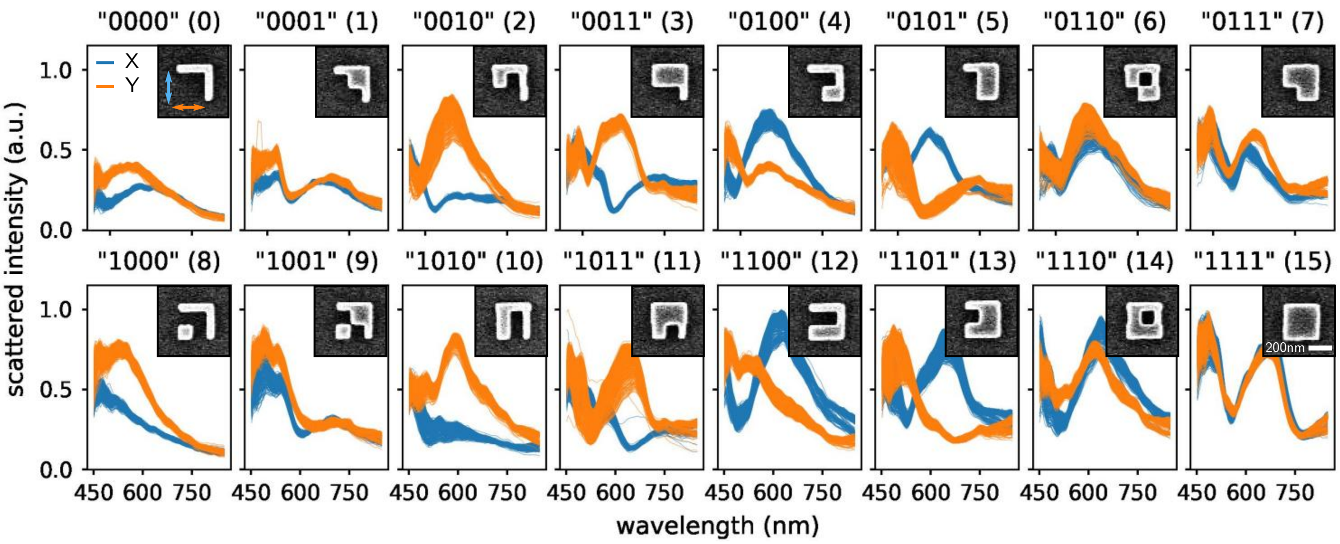


FIG. S.8. **Acquired spectra for 4 bit experimental datasets** Same as figure S.4 but for the 4 bit dataset.

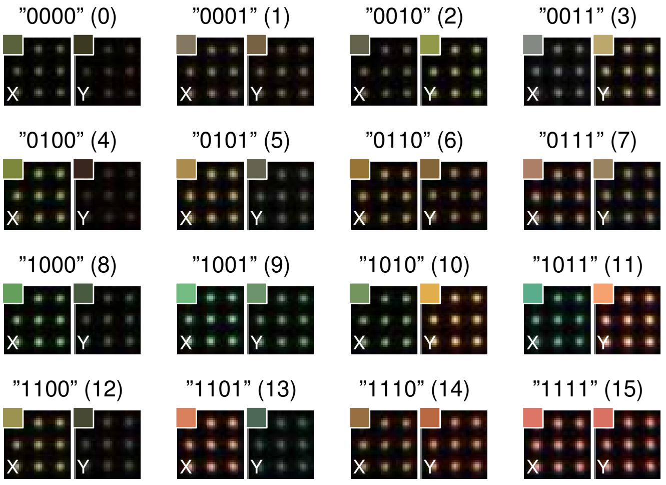


FIG. S.9. **DF microscopy image RGB color for 4 bit structures** Same as figure S.5, but for the 4 bit structures.

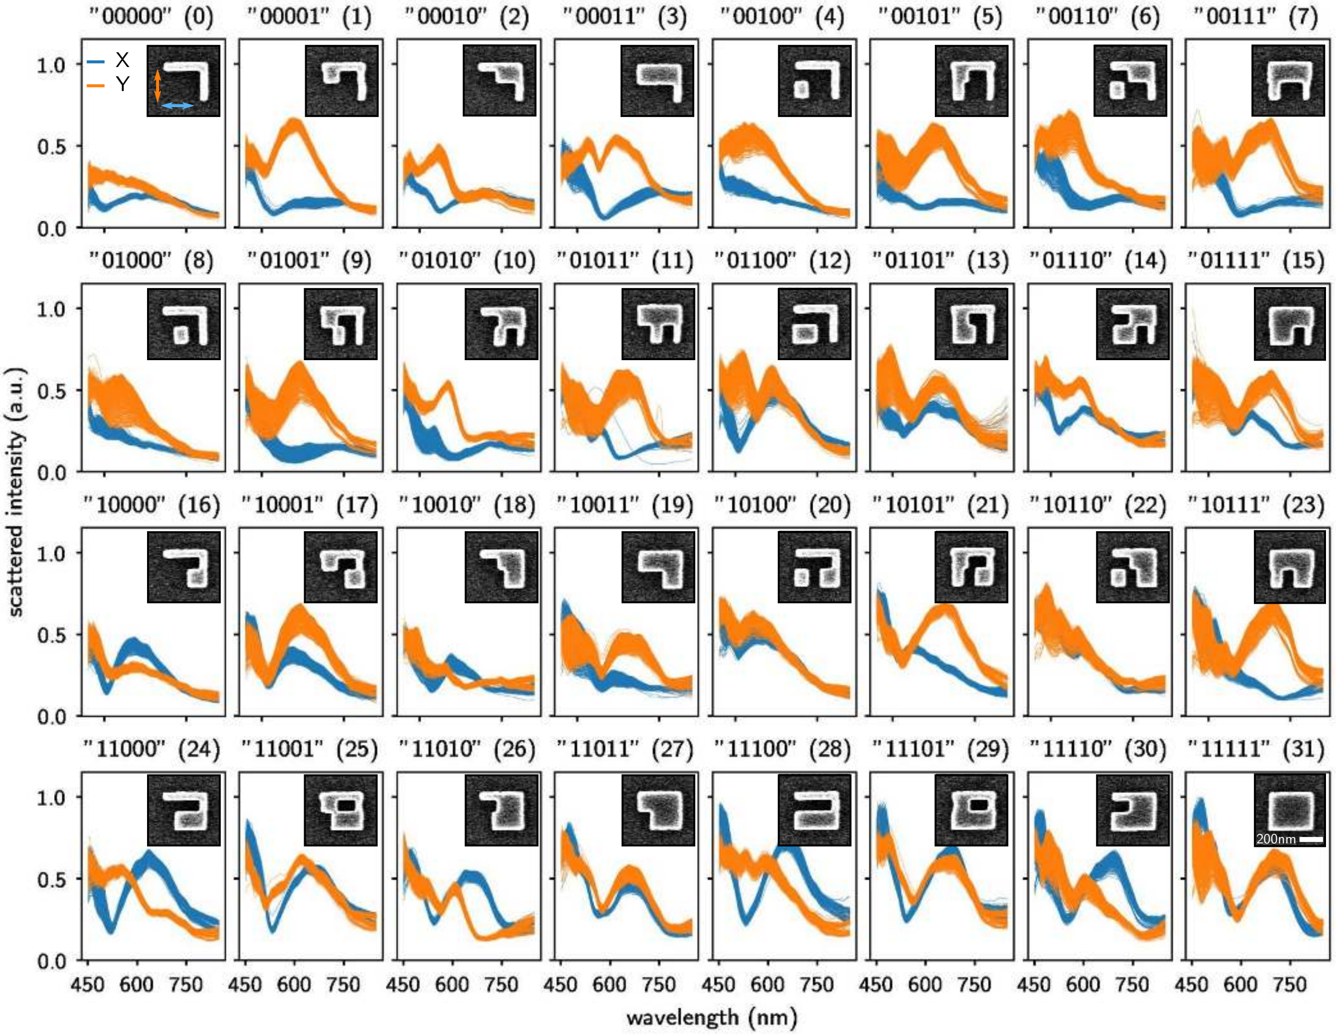


FIG. S.10. **Acquired spectra for 5 bit experimental datasets** Same as figure S.4 but for the 5 bit dataset.

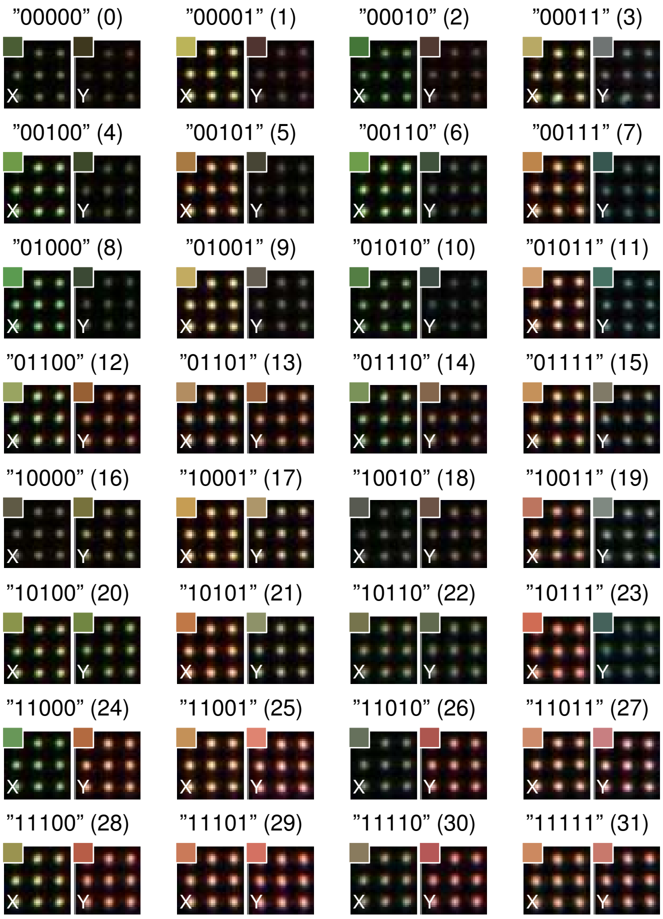


FIG. S.11. **DF microscopy image RGB color for 5 bit structures** Same as figure S.5, but for the 5 bit structures.

## III. REPRODUCIBILITY WITH SECOND 4-BIT SET, COMPARISON TO SIMULATIONS

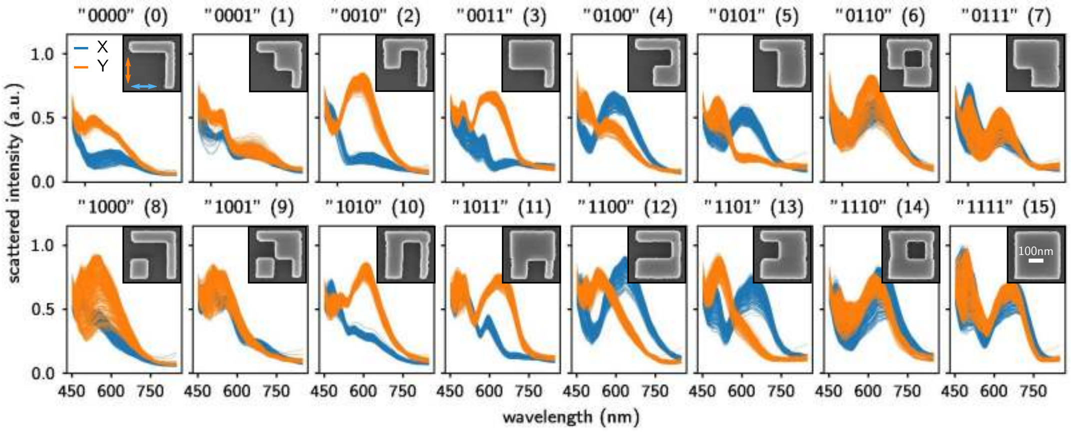


FIG. S.12. **Second set of 4 bit experimental structures** Scattering spectra from a second set of 4 bit encoding structures (575 copies of each geometry), fabricated and measured several months prior to the data shown in figure S.8. Read-out accuracy is similar to the newer dataset, with error-free operation using full spectra and similar performance in the RGB scheme (see figure S.13) While the spectra used for the results shown in the main text were measured at an acquisition time of $t_a = 0.2\,\mathrm{s}$, the alternative set was measured with $t_a = 0.5\,\mathrm{s}$. We assume that even shorter acquisition times would be sufficient for a robust recognition.

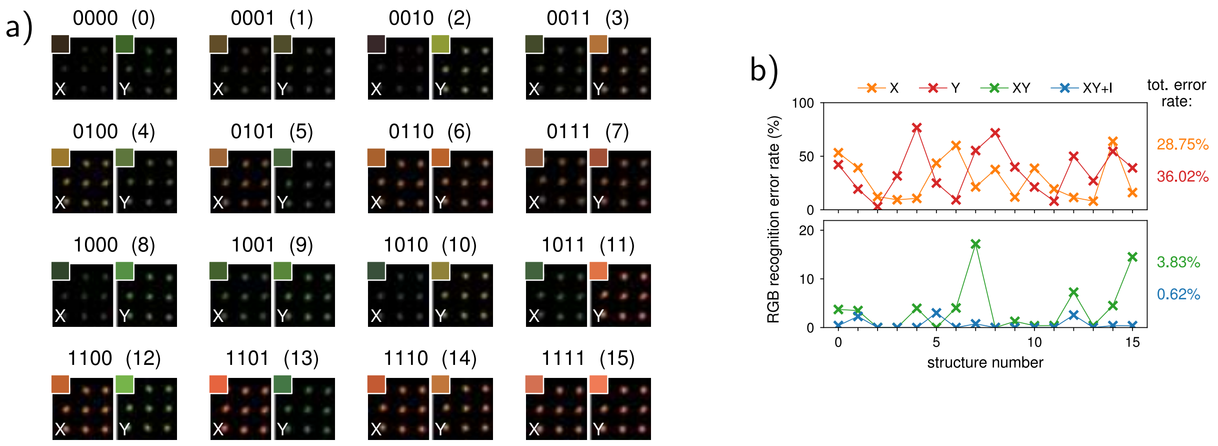


FIG. S.13. **RGB readout with second 4 bit dataset** a) RGB color from polarized DF microscopy images for 9 selected copies of each structure. The color-box inset at the top right corresponds to the average RGB color of the shown structures (c.f. figure S.9). b) same as figure S.16 but based on the second set of 4 bit structures, fabricated and measured several months earlier.

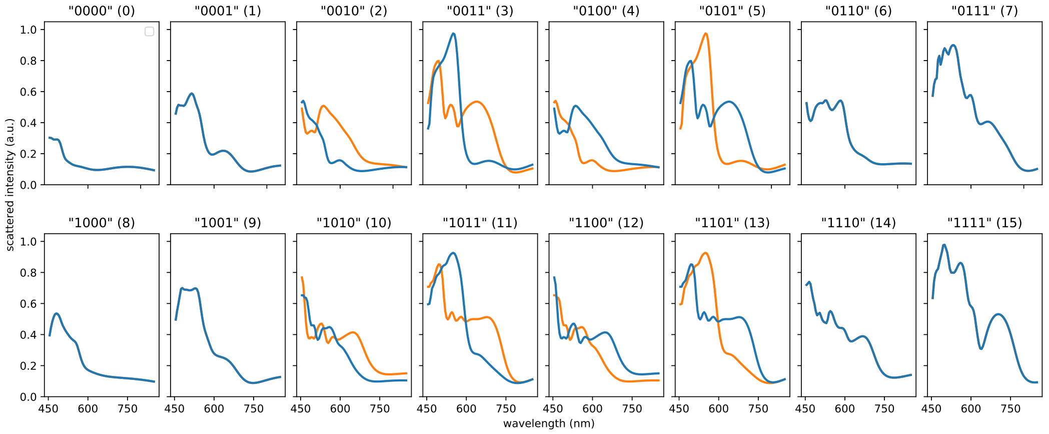


FIG. S.14. **Simulated spectra for the 4 bit** Simulated intensity of backscattered light for the structures encoding 4bit of information. SEM images are $385 \times 385\,\mathrm{nm}^2$ large, scalebar in "1111" is 100 nm.

## IV. T-SNE PLOTS FOR ALL DATASETS

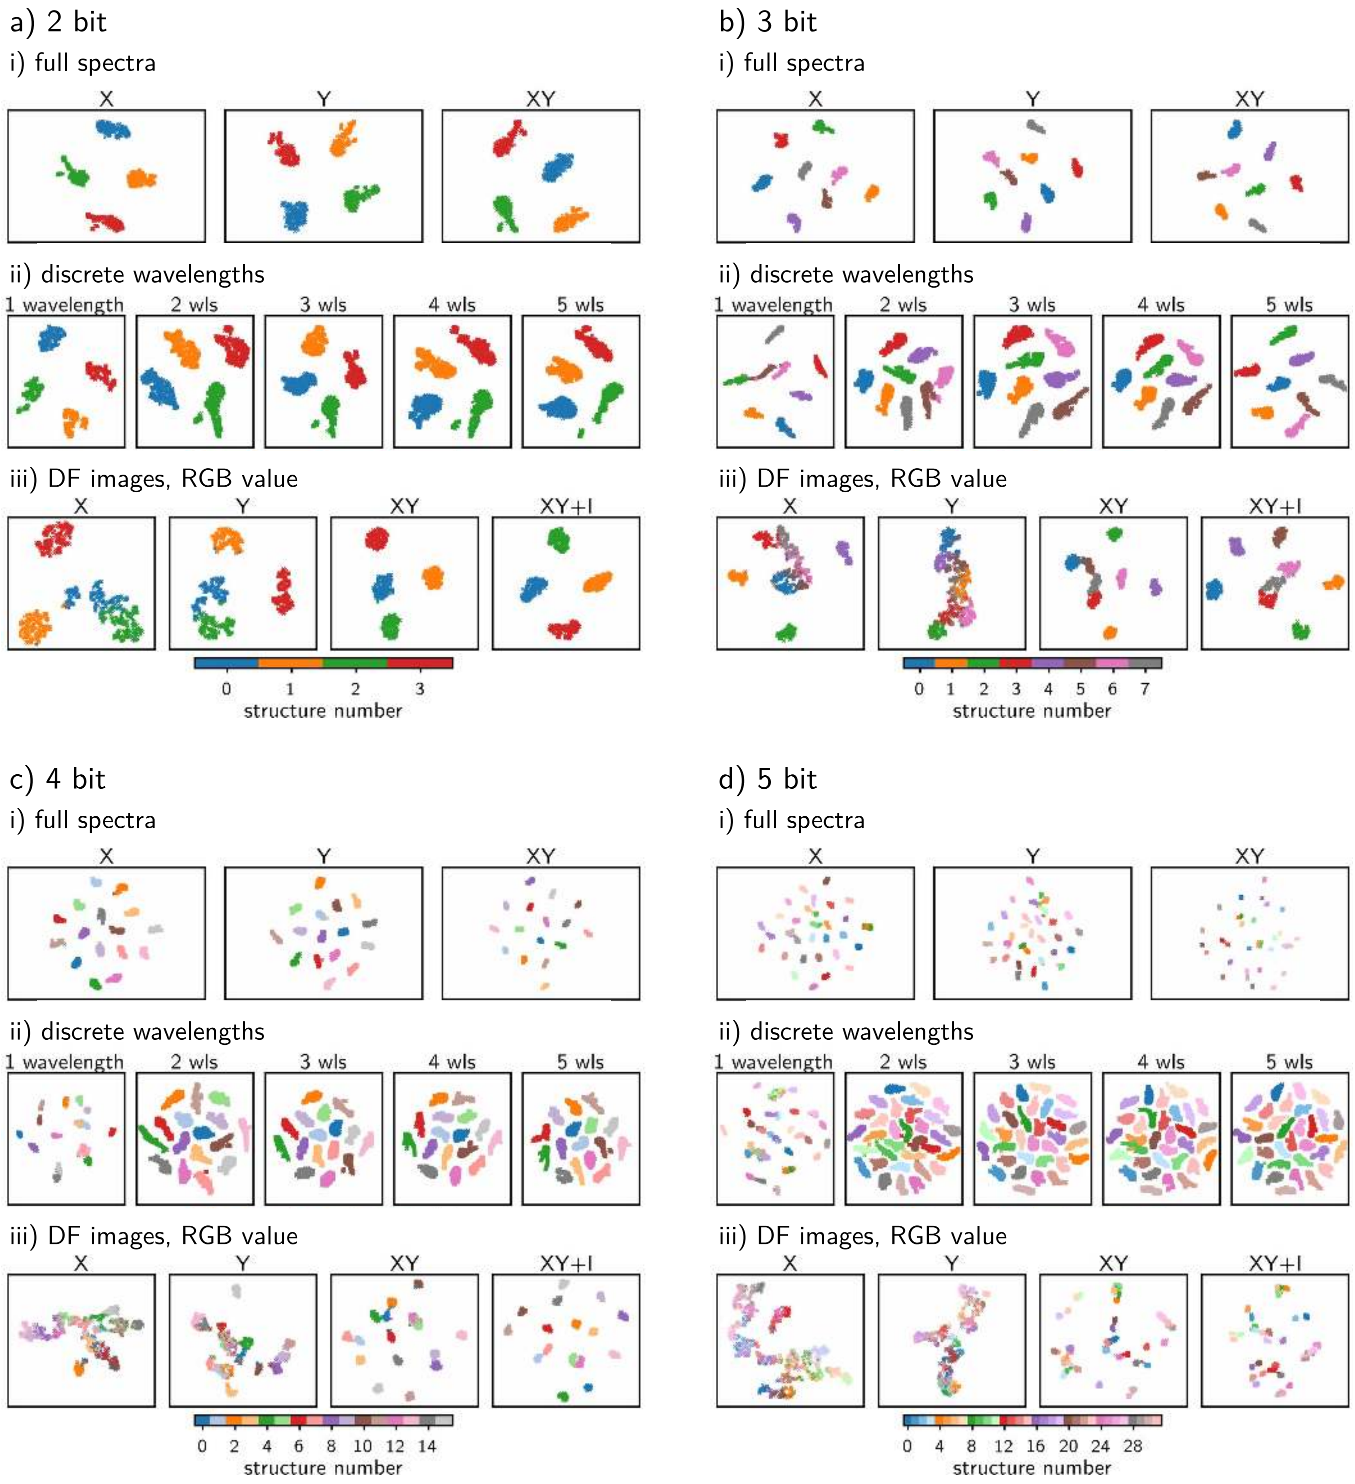


FIG. S.15. **t-SNE plots for all experimental datasets** a) 2 bit, b) 3 bit, c) 4 bit and d) 5 bit. Each bit-density contains t-SNE evaluations for (i) the full spectra, (ii) a fixed number of discrete wavelengths and (iii) the darkfield image RGB values.

## V. ERROR RATES FOR EACH BIT-SEQUENCE IN THE RGB READ-OUT MODEL

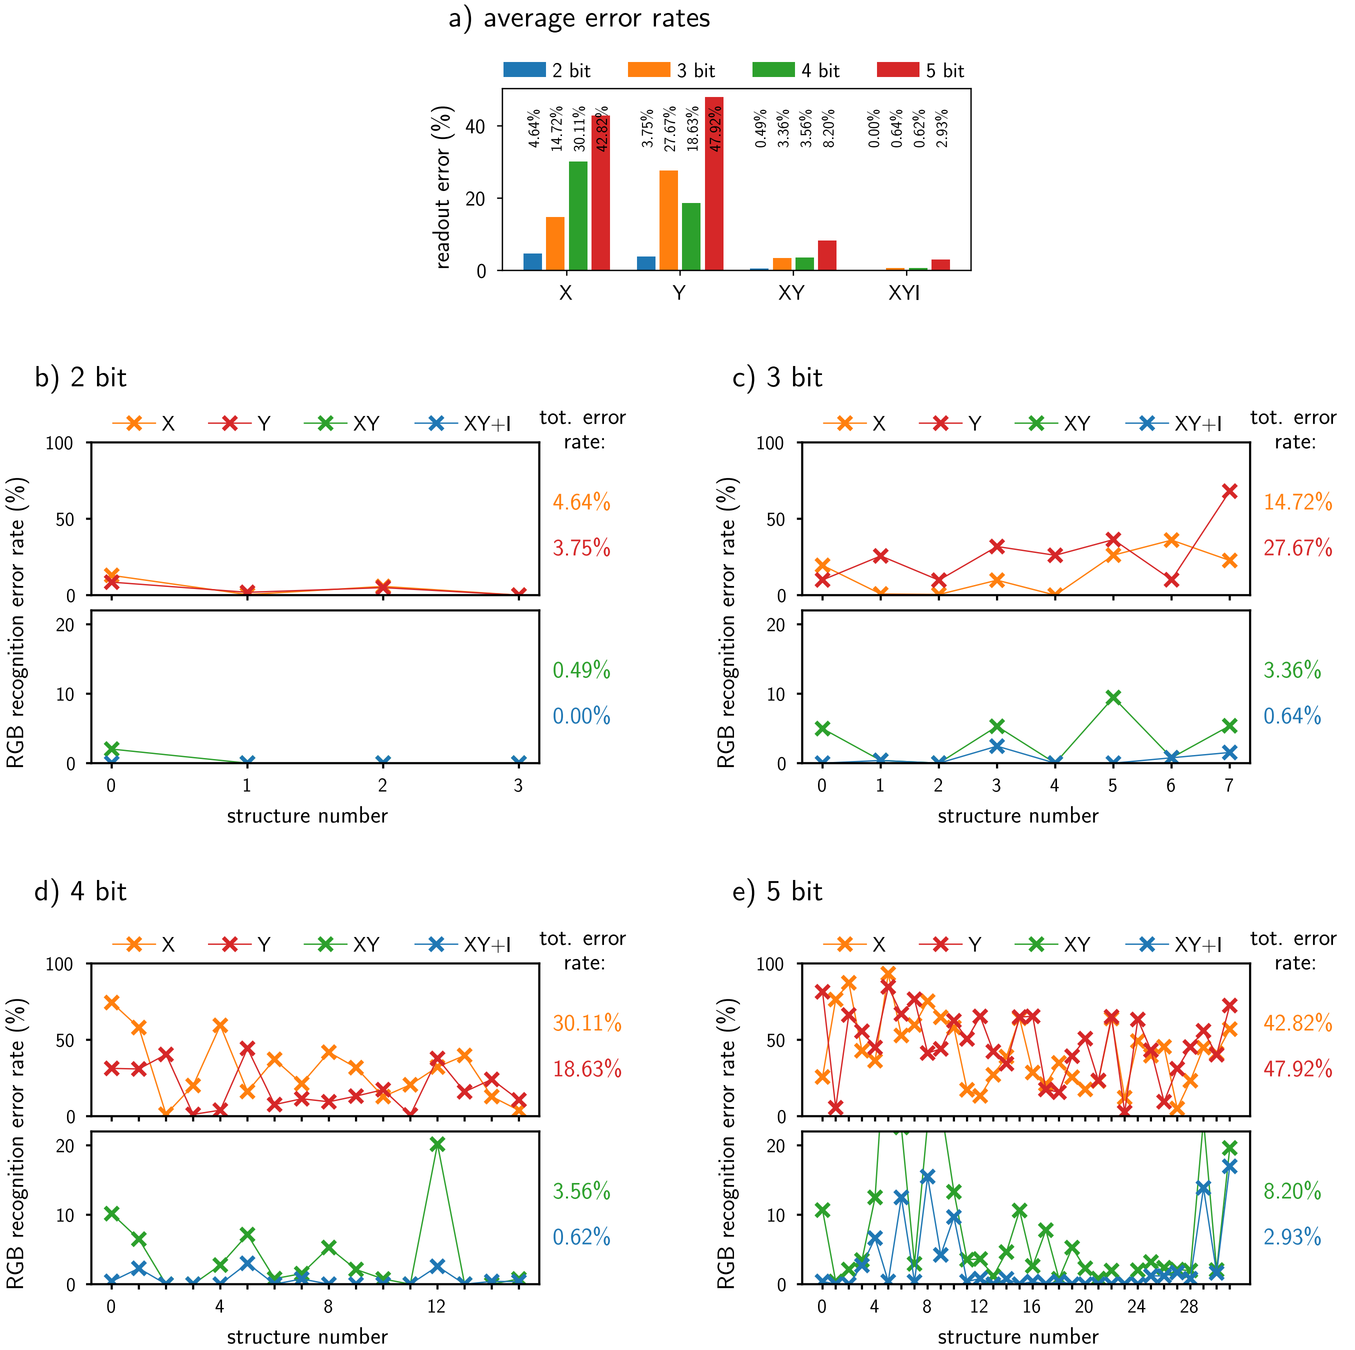


FIG. S.16. **Error rates for each bit-sequence using the RGB DF microscopy read-out scheme.** a) Average read-our error for the different datasets (reproduced from figure 5, main text). b-e) retrieval error rate for each encoded bit sequence for the b) 2 bit, c) 3bit, d) 4 bit and e) 5 bit datasets. The efficiency of read-out is assessed for different subsets of the full data: only $X$ polarized images (orange), only $Y$ polarization (red), both $X$ and $Y$ polarizations (green), and using as well the scattering intensity (blue lines).

## VI. SOFTMAX OUTPUT LAYER OF THE NEURAL NETWORK ON THE RGB DATA

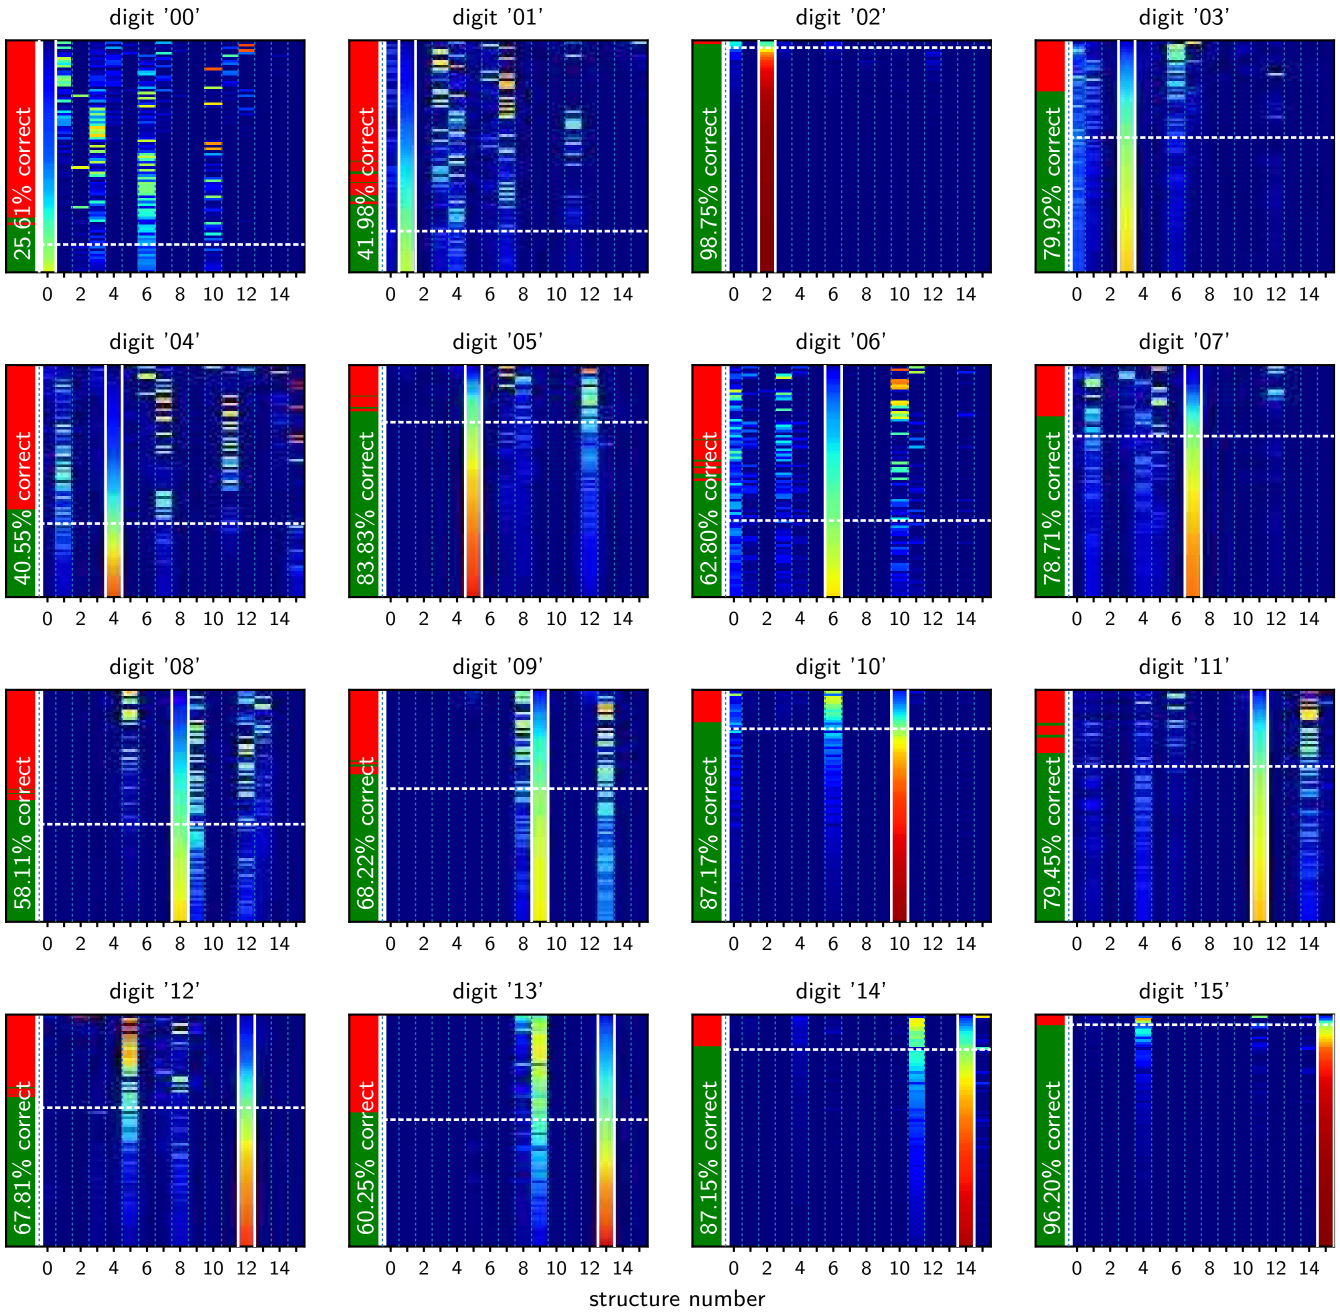


FIG. S.17. **Activations of the softmax output layer neurons on the 4 bit RGB-"X" validation dataset.** Each subplot corresponds to all input data for a specific digit (see text above the subplots). The correct digit is highlighted by white vertical bars. The datasets are sorted by the level of activation of the neuron corresponding to the correct digit (bottom: highest, top: lowest activation). An activation of 0.5 is indicated by a dashed white horizontal line. A bar on the left indicates, whether the structure has been correctly identified (green) or not (red).

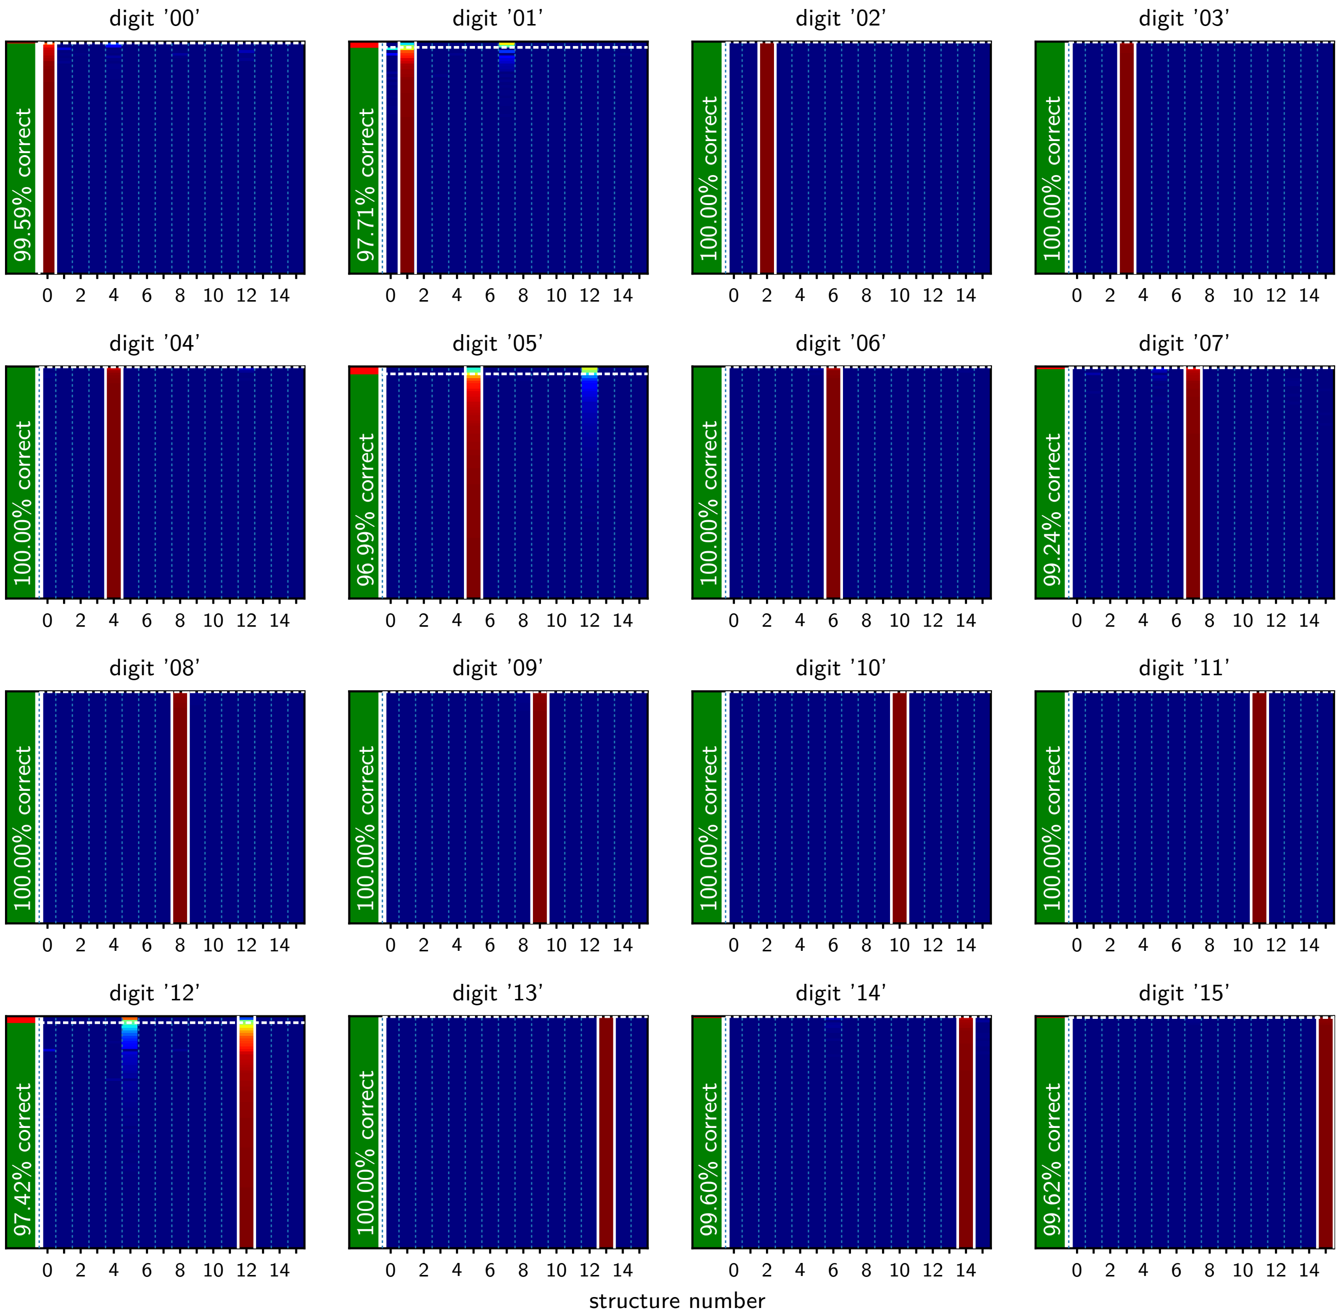


FIG. S.18. **Activations of the softmax output layer neurons on the 4 bit RGB-"XY+I" validation dataset.** Same as figure S.17 but for the RGB-"XY+I" dataset.

## VII. EMBEDDING IN $SIO_2$

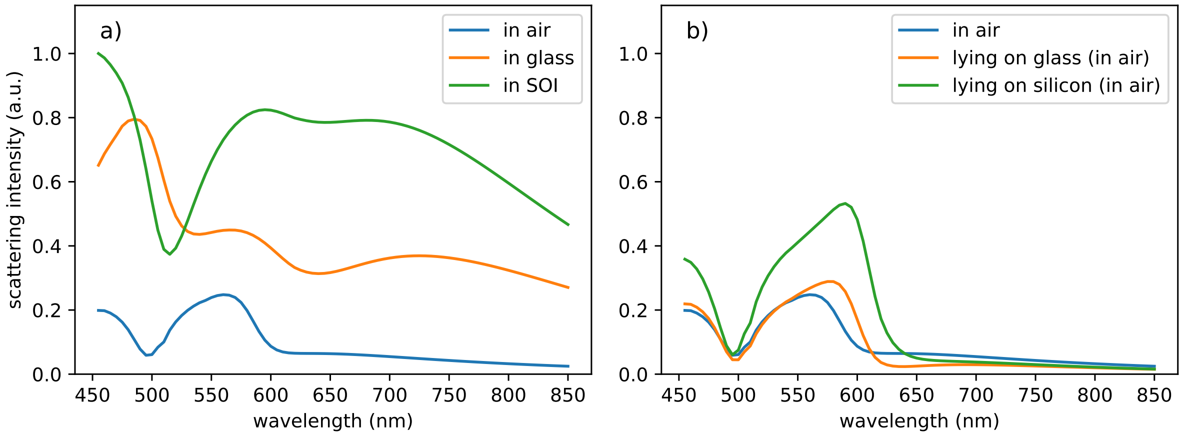


FIG. S.19. **Numerical assessment of influence of nanostructure environment** Numerical comparison of backscattering intensity from a plane wave illuminated silicon cuboid ($160 \times 160 \times 120\,\mathrm{nm}^3$). a) embedded in bulk $SiO_2$ (orange line) or in $SiO_2$, 30 nm above a silicon substrate ("SOI", green line). Embedding the silicon structure in a medium of $n > 1$ not only causes a red-shift and a broadening of the resonances, but can even entirely perturb the general shape of the spectra. b) comparison of substrates: in air, the scattering resonances mainly red-shift and broaden with increasing substrate refractive index. The global form of the spectra is generally conserved. The green line in a) ("SOI") corresponds to the conditions used in our experiments. Compared to lying on the $SiO_2$ layer in air, a distinctly stronger back-scattering can be expected in case of the SOI substrat with an embedding $SiO_2$ layer on top. Data globally normalized to the same scale.

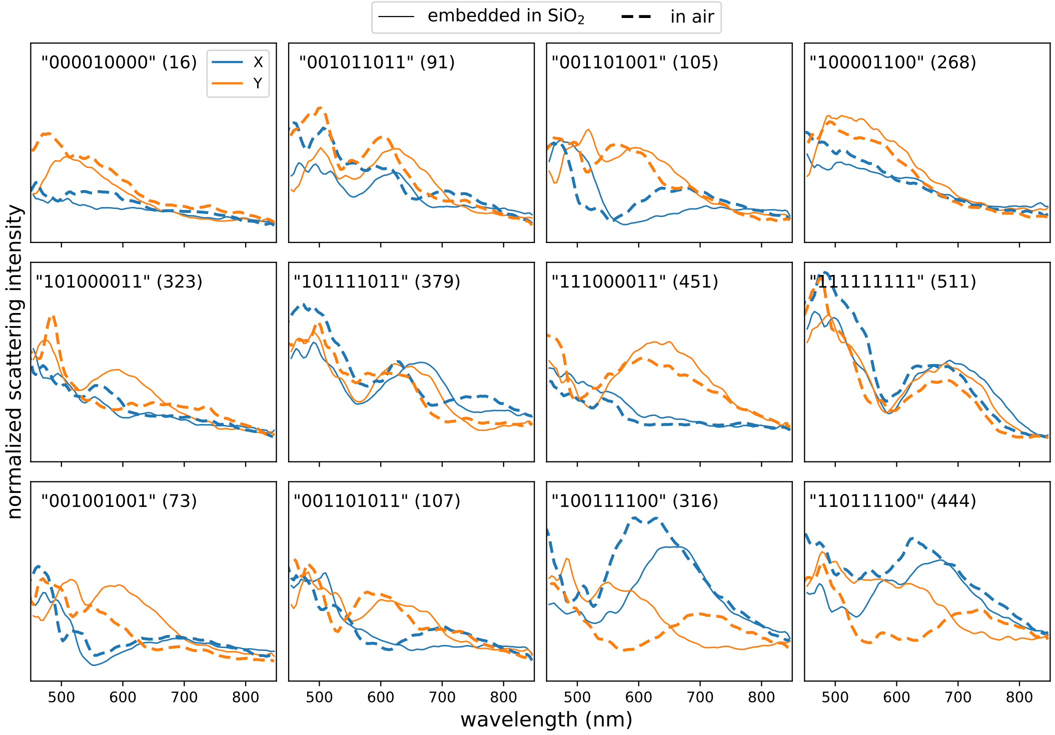


FIG. S.20. **Experimental analysis of the impact of embedding the structures in $SiO_2$** Experimental comparison of backscattering spectra from selected "9 bit" structures, fabricated on top of the bare SOI substrate (dashed lines) and for the same structures embedded inside an additional $SiO_2$ deposited layer (thin solid lines). The incident light is polarized along $X$ (blue) or along $Y$ (orange). The resonances are red-shifted in case of the surrounding $SiO_2$, which also induces some broadening due to damping. Interestingly, in contrast to what we expect from the simulations shown in figure S.19, the scattering intensity is comparably strong in both cases. We attribute this to higher than expected absorption in the deposited $SiO_2$ layer, whose quality is probably not perfect. Studying the optical properties of our deposited $SiO_2$ is however beyond the scope of the present work.

## VIII. 9 BIT STRUCTURES – ASSESSING THE EXPERIMENTAL FEASIBILITY

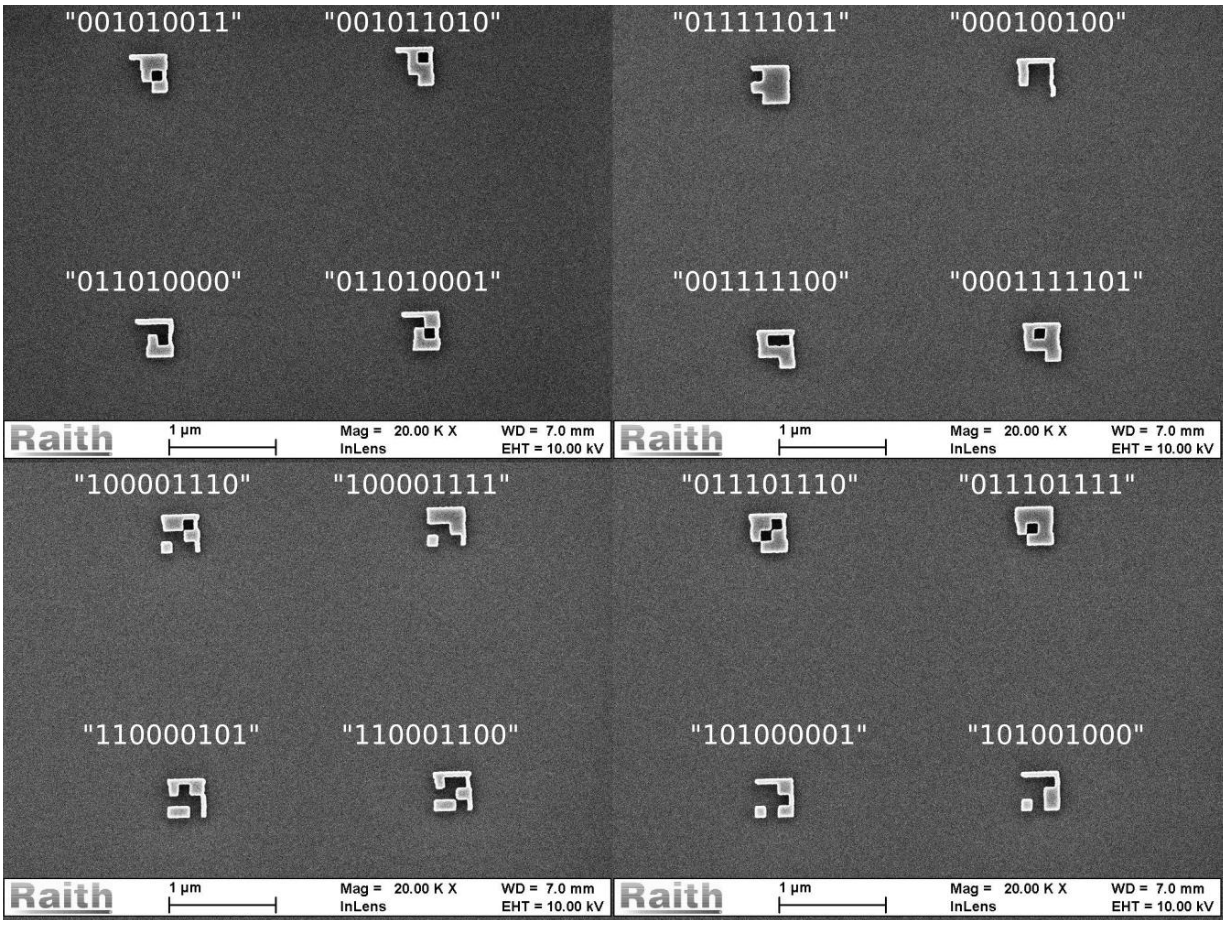


FIG. S.21. **Selected SEM images of fabricated 9-bit encoding structure set** We fabricated 4 copies of the full 9-bit set of structures (512 different structures required to encode sequences of 9 bits). Here we show some selected SEM images. The fabrication quality of all structures is equally good as in the examples shown here. Scale bars are 1 µm.

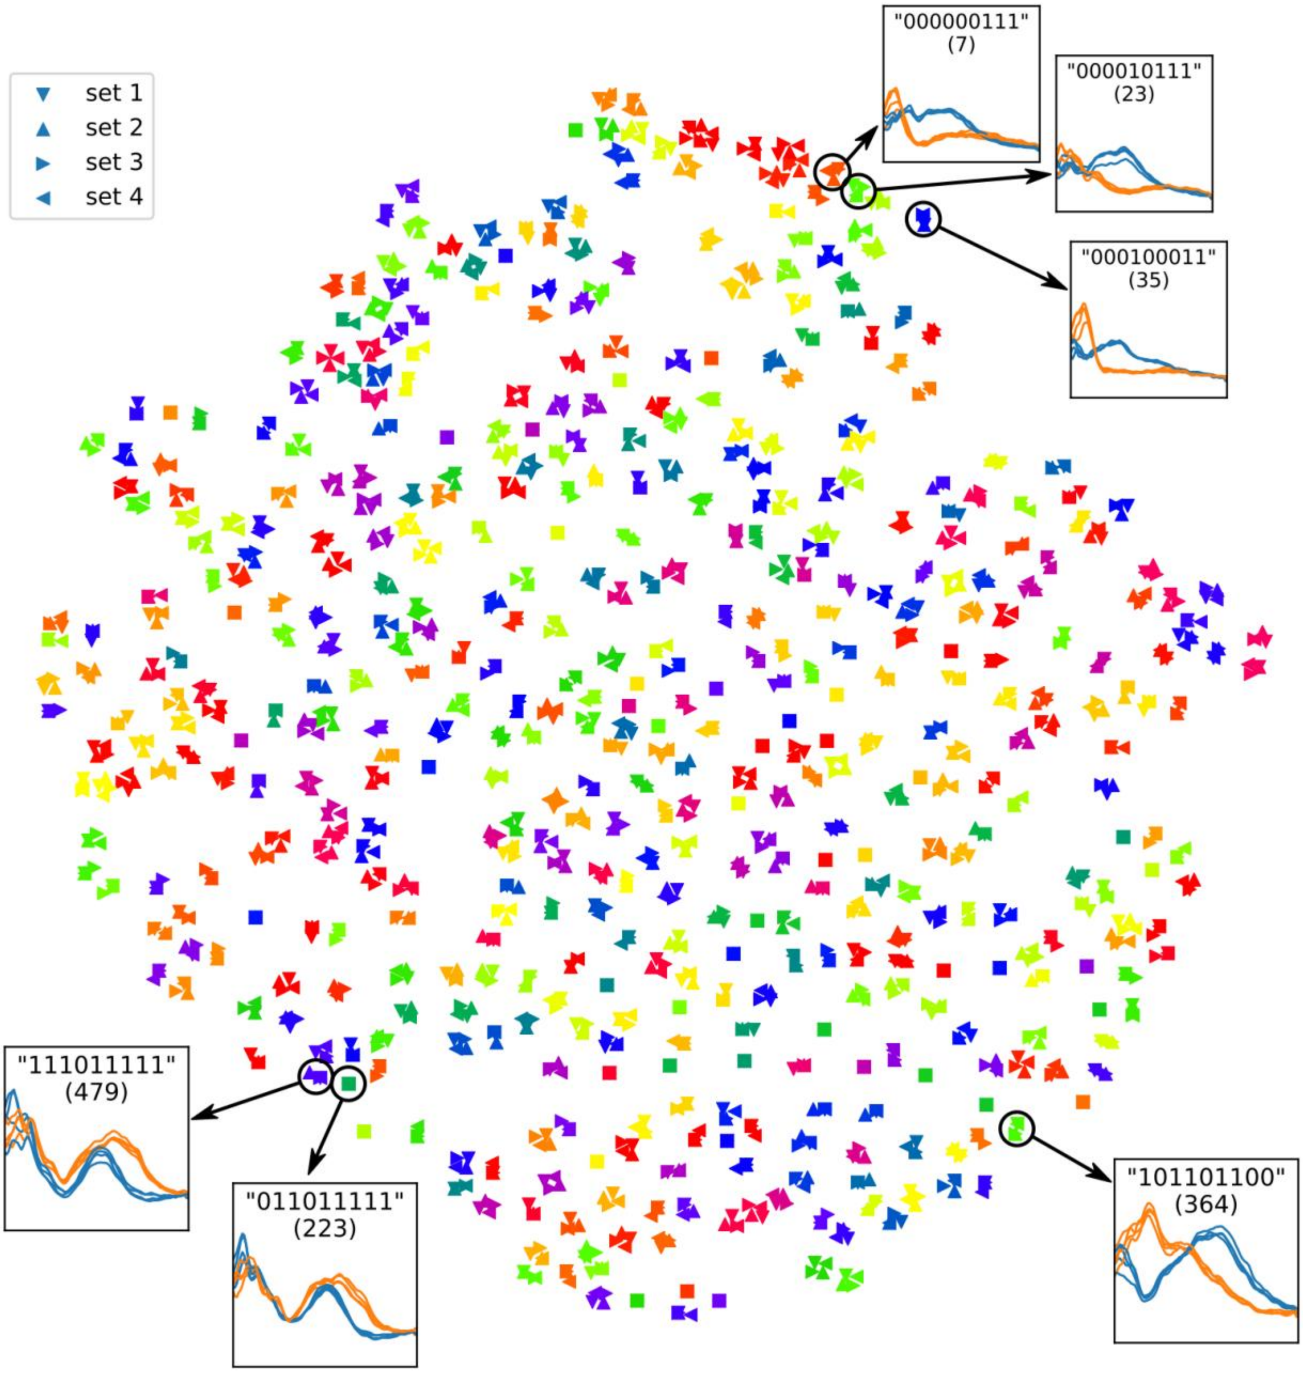


FIG. S.22. **Experimental spectra "t-SNE" analysis of the 9 bit structures** Each point corresponds to a measured spectrum of a 9-bit nanostructure. Four copies of each of the 512 different structures were fabricated and are shown here. Each color corresponds to a geometry of a different bit-sequence. In order to be well distinguishable spectra, points have to be well separated in the t-SNE plot. Different structures are indeed mostly well separated in the plot, while the four identical copies (set 1-4: left, right, top and bottom markers) are more or less superposed. Insets show selected spectra, corresponding to the highlighted markers in the plot.

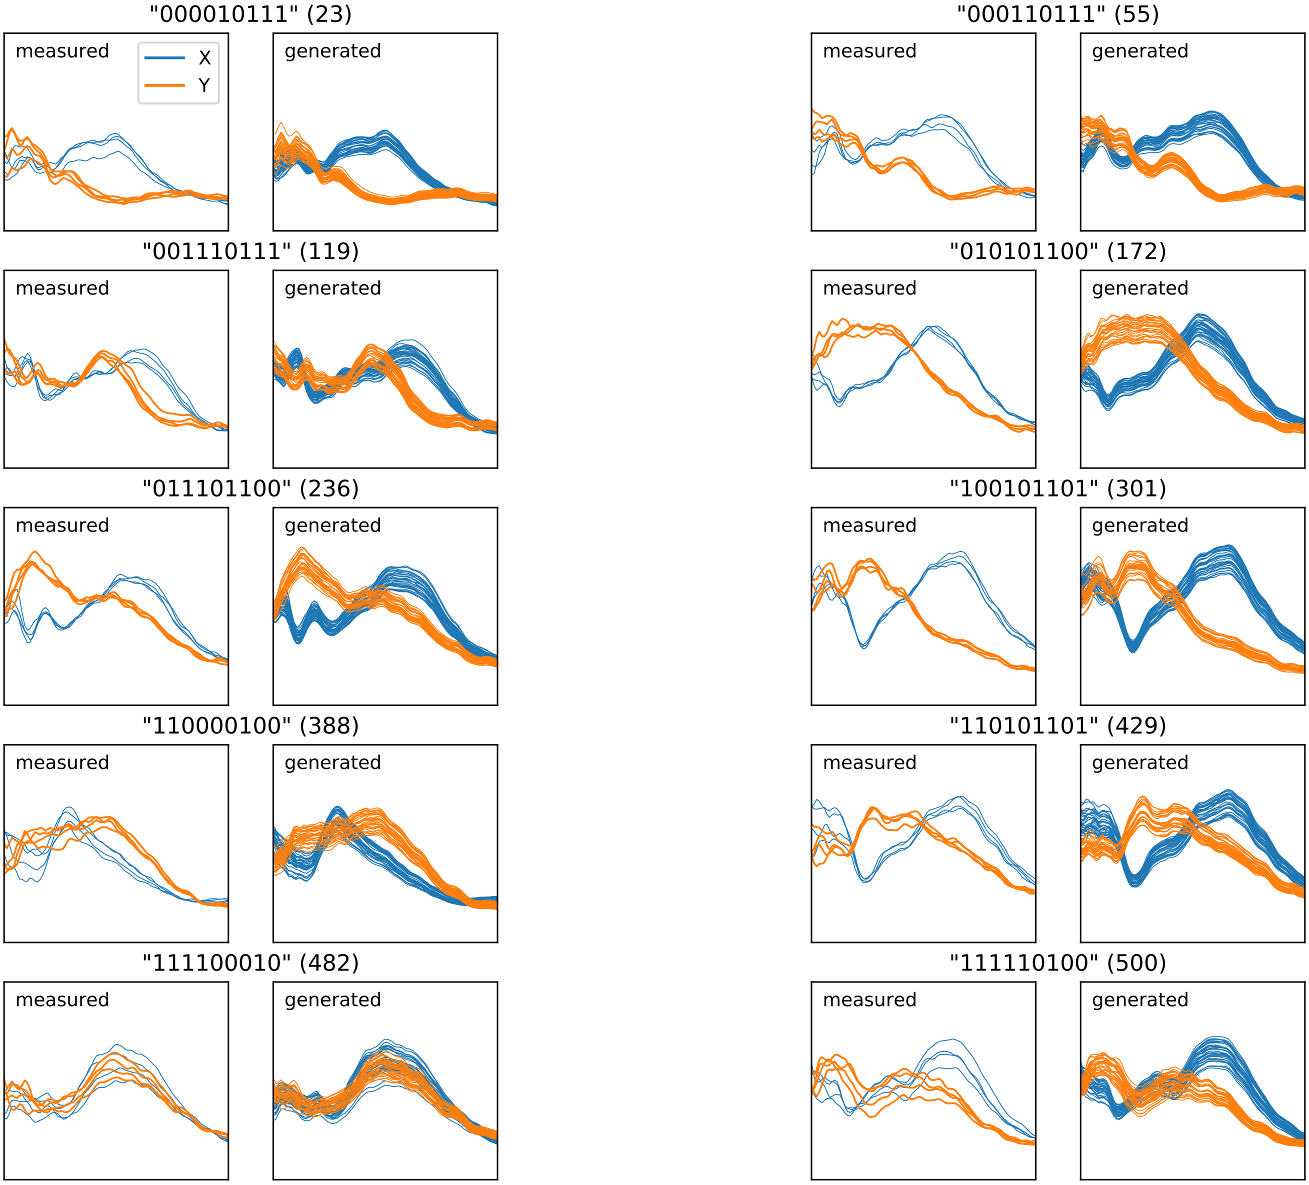


FIG. S.23. **Generation of experimental 9 bit training dataset from measured spectra** Measured spectra (left subplots) and network training data generated from the experimental data (right subplots) for selected geometries of the 9-bit structures. The generated data is a random superposition of the four measured spectra for each geometry, multiplied times a random scaling factor, which can increase or decrease the total intensity by up to 10 % of the original value.

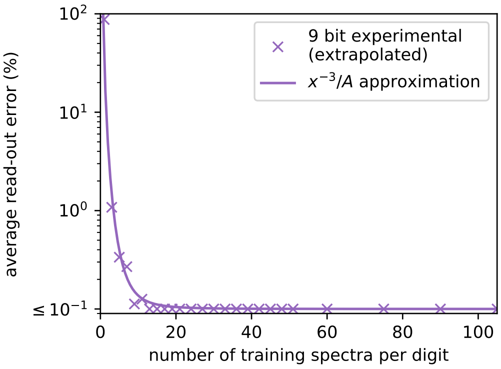


FIG. S.24. **Accuracy vs. training set size for 9 bit experimental training-set** Training convergence of experimental expanded 9 bit set as function of training samples per digit. The accuracy improves faster than expected, which we attribute to a lower variance in the expanded 9 bit spectra (which are based on only 4 measurements) compared to the 2-5 bit cases. The fully experimental sets for 2-5 bits contain more significant variations (resonance positions, intensity, noise, ...). The data is phenomenologically approximated by an $x^{-3}/A$ function (solid lines).

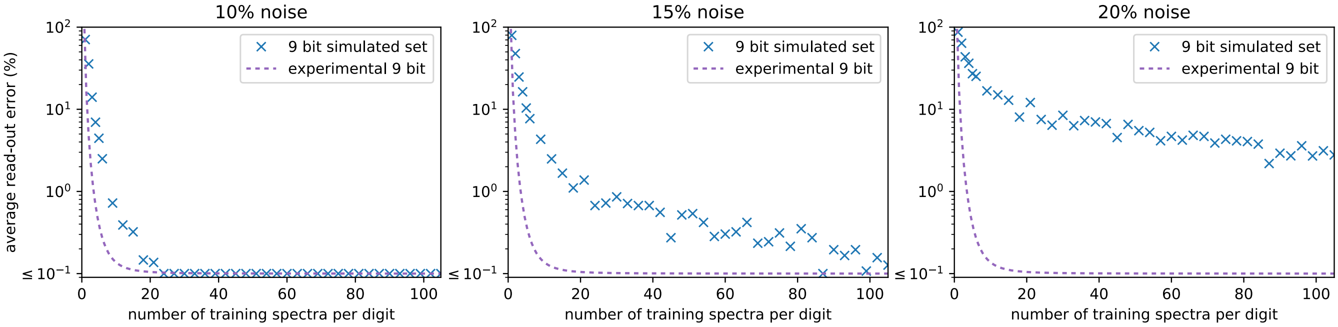


FIG. S.25. **Error rate as function of training batch size for the numerical 9-bit dataset** Read-out error as function of the training set size for the numerical 9-bit data with (a) 10%, (b) 15% and (c) 20% level of random noise. As also shown in main text figure 6, 15 % of noise correspond approximately to the limit, still allowing an accurate readout operation. The dashed line corresponds to the analytical approximation of the 9 bit experimental dataset training convergence (see Figure S.24).

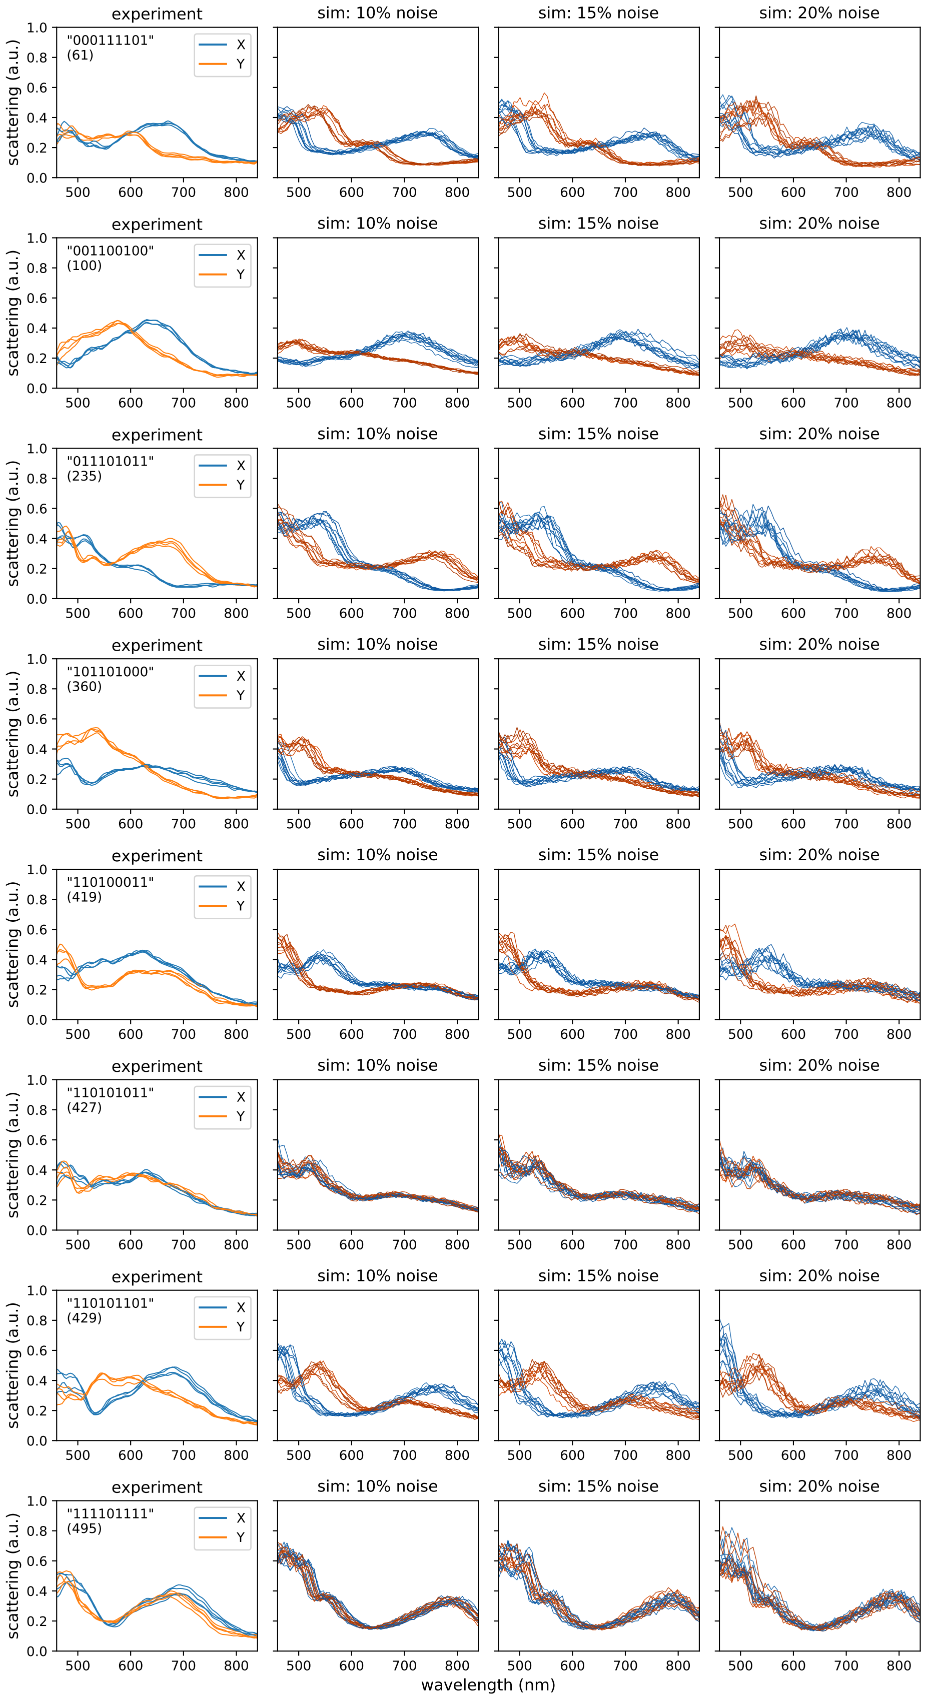


FIG. S.26. **Comparison of selected simulated and experimental 9-bit spectra** Experimental spectra obtained from 4 different copies of selected 9-bit encoding structures (left subplots) are compared to the corresponding simulated scattering spectra with different numerical noise levels. Each plot shows 10 randomly noised spectra for each polarization ($X$ blue, $Y$ orange lines). Second left subplot: 10 % noise, second right subplot: 15 % noise, right subplot: 20 % noise. Structures 427 and 495 are symmetric. The reproducibility of the experimental spectra seems to be clearly better than in the 15 % noise numerical dataset. Training on the 15 % noise numerical dataset still yields almost error-free read-out in the order of 99.9 % accuracy. We conclude that experimental 9bit density should be feasible.

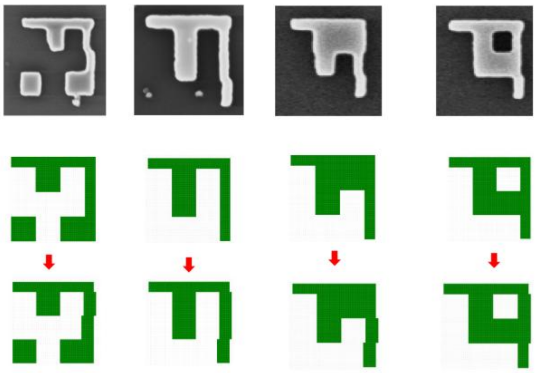

FIG. S.27. **Manual correction scheme for non-symmetric fabrication distortions** Illustration how the fabricational asymmetry between $X$- and $Y$-orientated features can be manually corrected at the level of the lithographic mask.

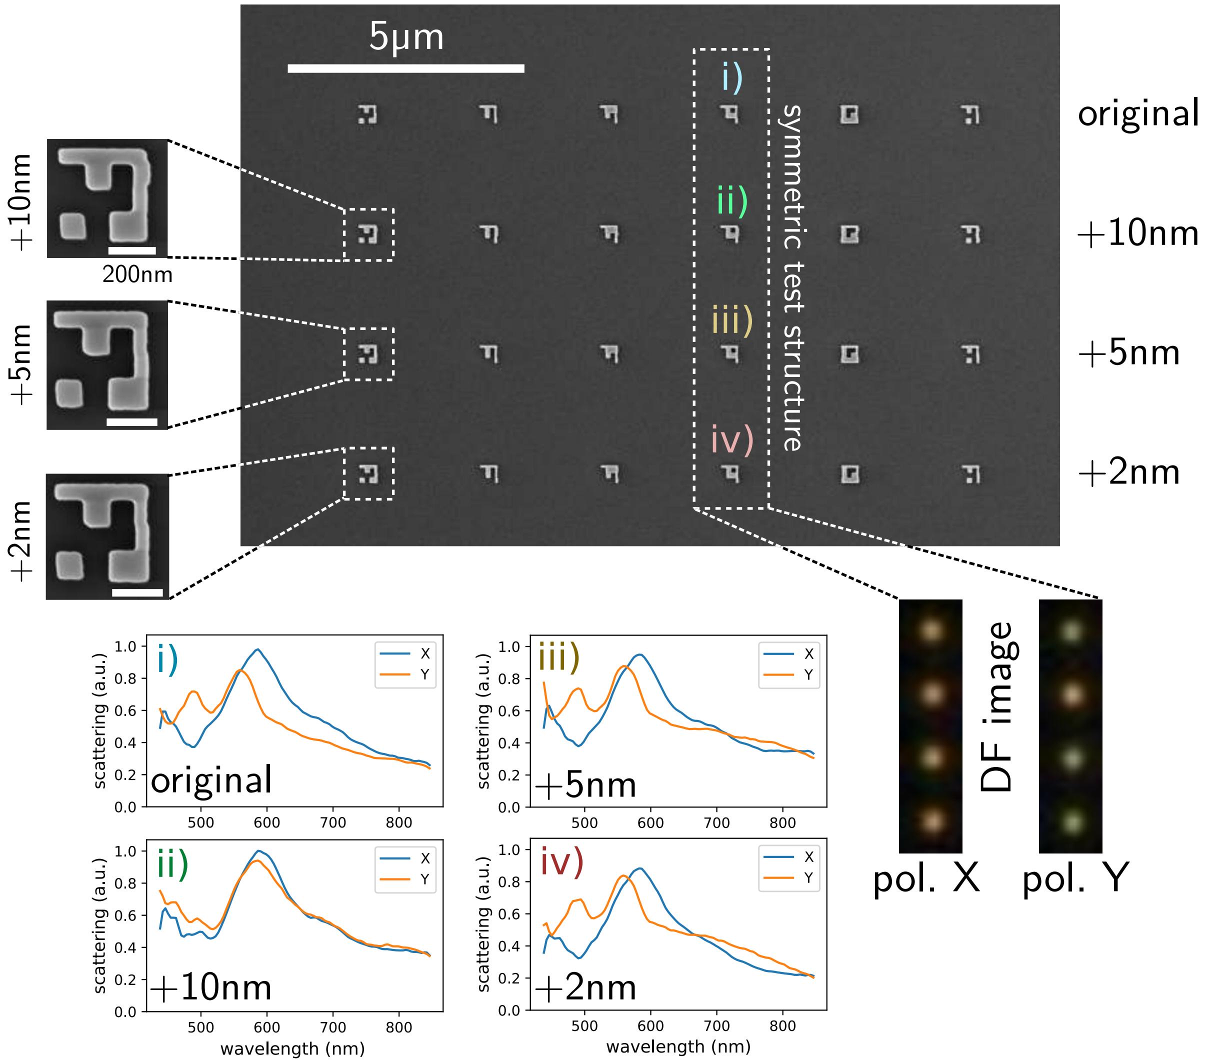


FIG. S.28. **Correction for non-symmetric fabrication distortions** SEM images of symmetry-corrected structures with different large correction widths. Bottom: Experimental scattering spectra (left) of the symmetric test structure with different correction widths and corresponding polarization filtered DF images (right). In conclusion, the fabrication-process inherent asymmetry can be effectively accounted for using an accordingly adapted lithographic mask. The optimum correction width seems to lie somewhere close to 10 nm, which can be applied in an automated way during the mask-generation. However, we note that for our digital information storage application, the observed asymmetries don't pose a problem, since the deep neural network will learn the retrieval of the data from the actual optical response of the fabricated structures, and does not rely on numerical simulations of idealized geometries. Such asymmetries might even be advantageous since they increase the "uniqueness" of the different structures and their scattering spectra.

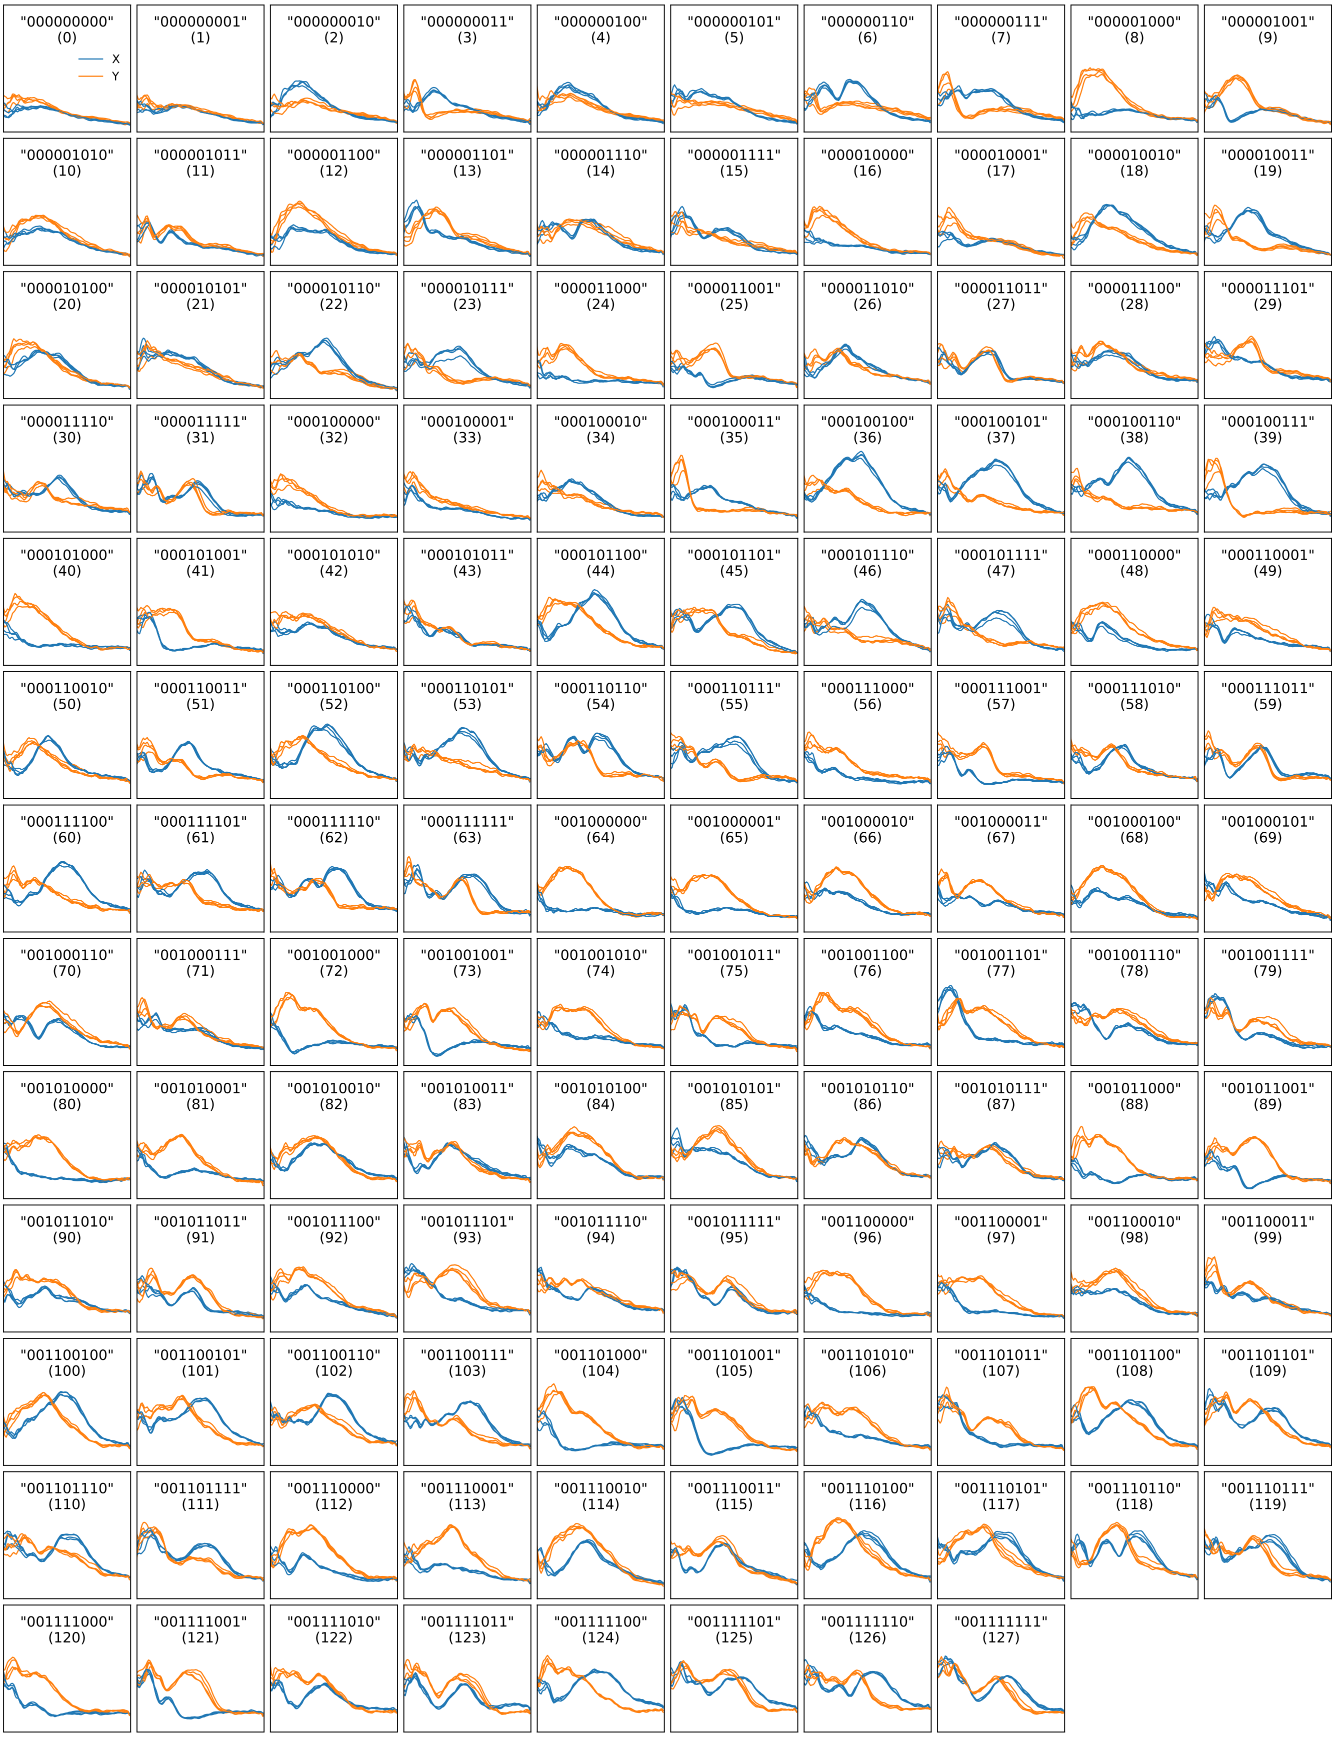


FIG. S.29. **Experimental spectra for the 9 bit structures 1/4** First 128 structures of spectra of all 9 bit encoding structures. We fabricated and measured four different copies of each structure, demonstrating the excellent reproducibility of the measurements. All spectra are plotted on the same $Y$ scale and show a spectral range from 450 nm to 850 nm.

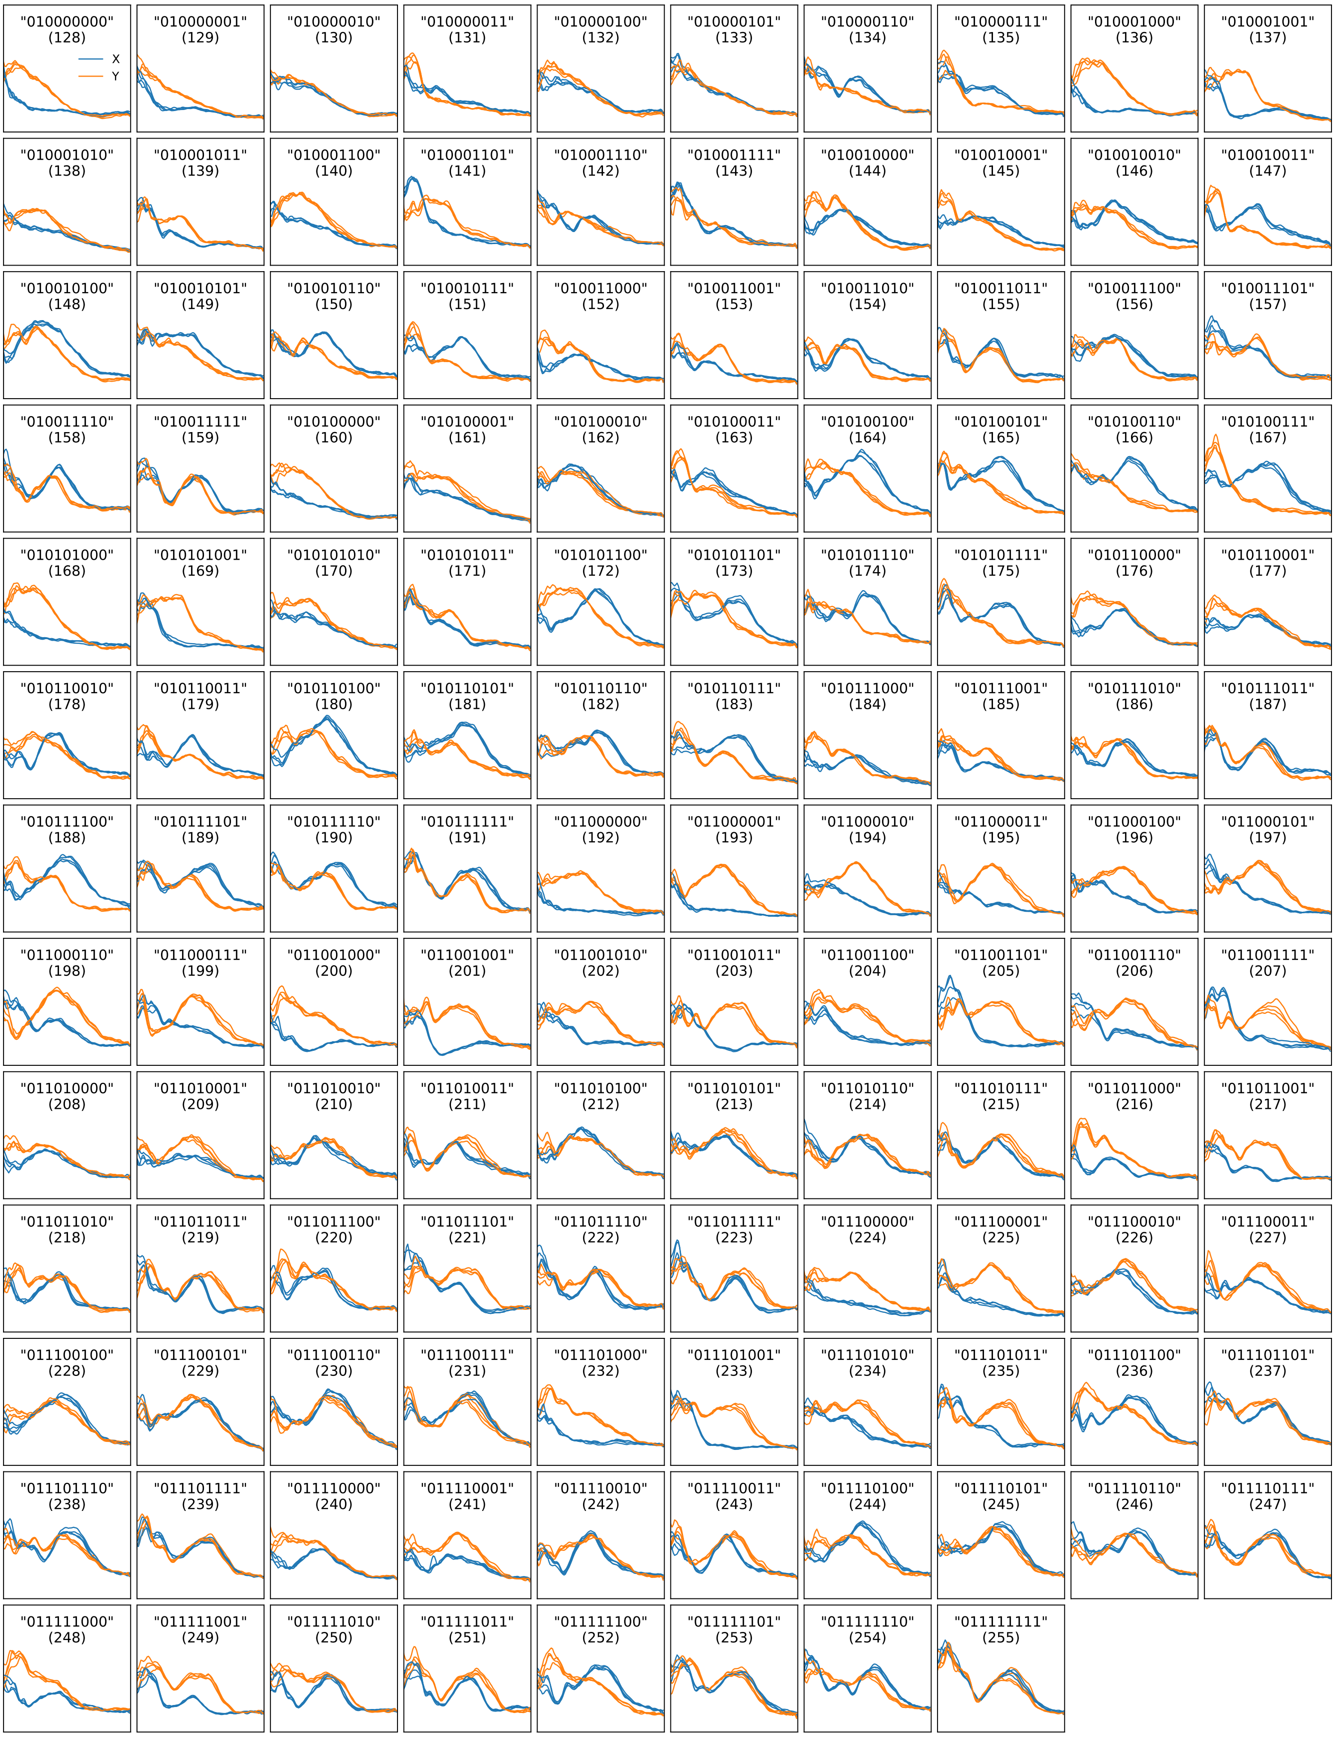


FIG. S.30. **Experimental spectra for the 9 bit structures 2/4** Structures 127-255.

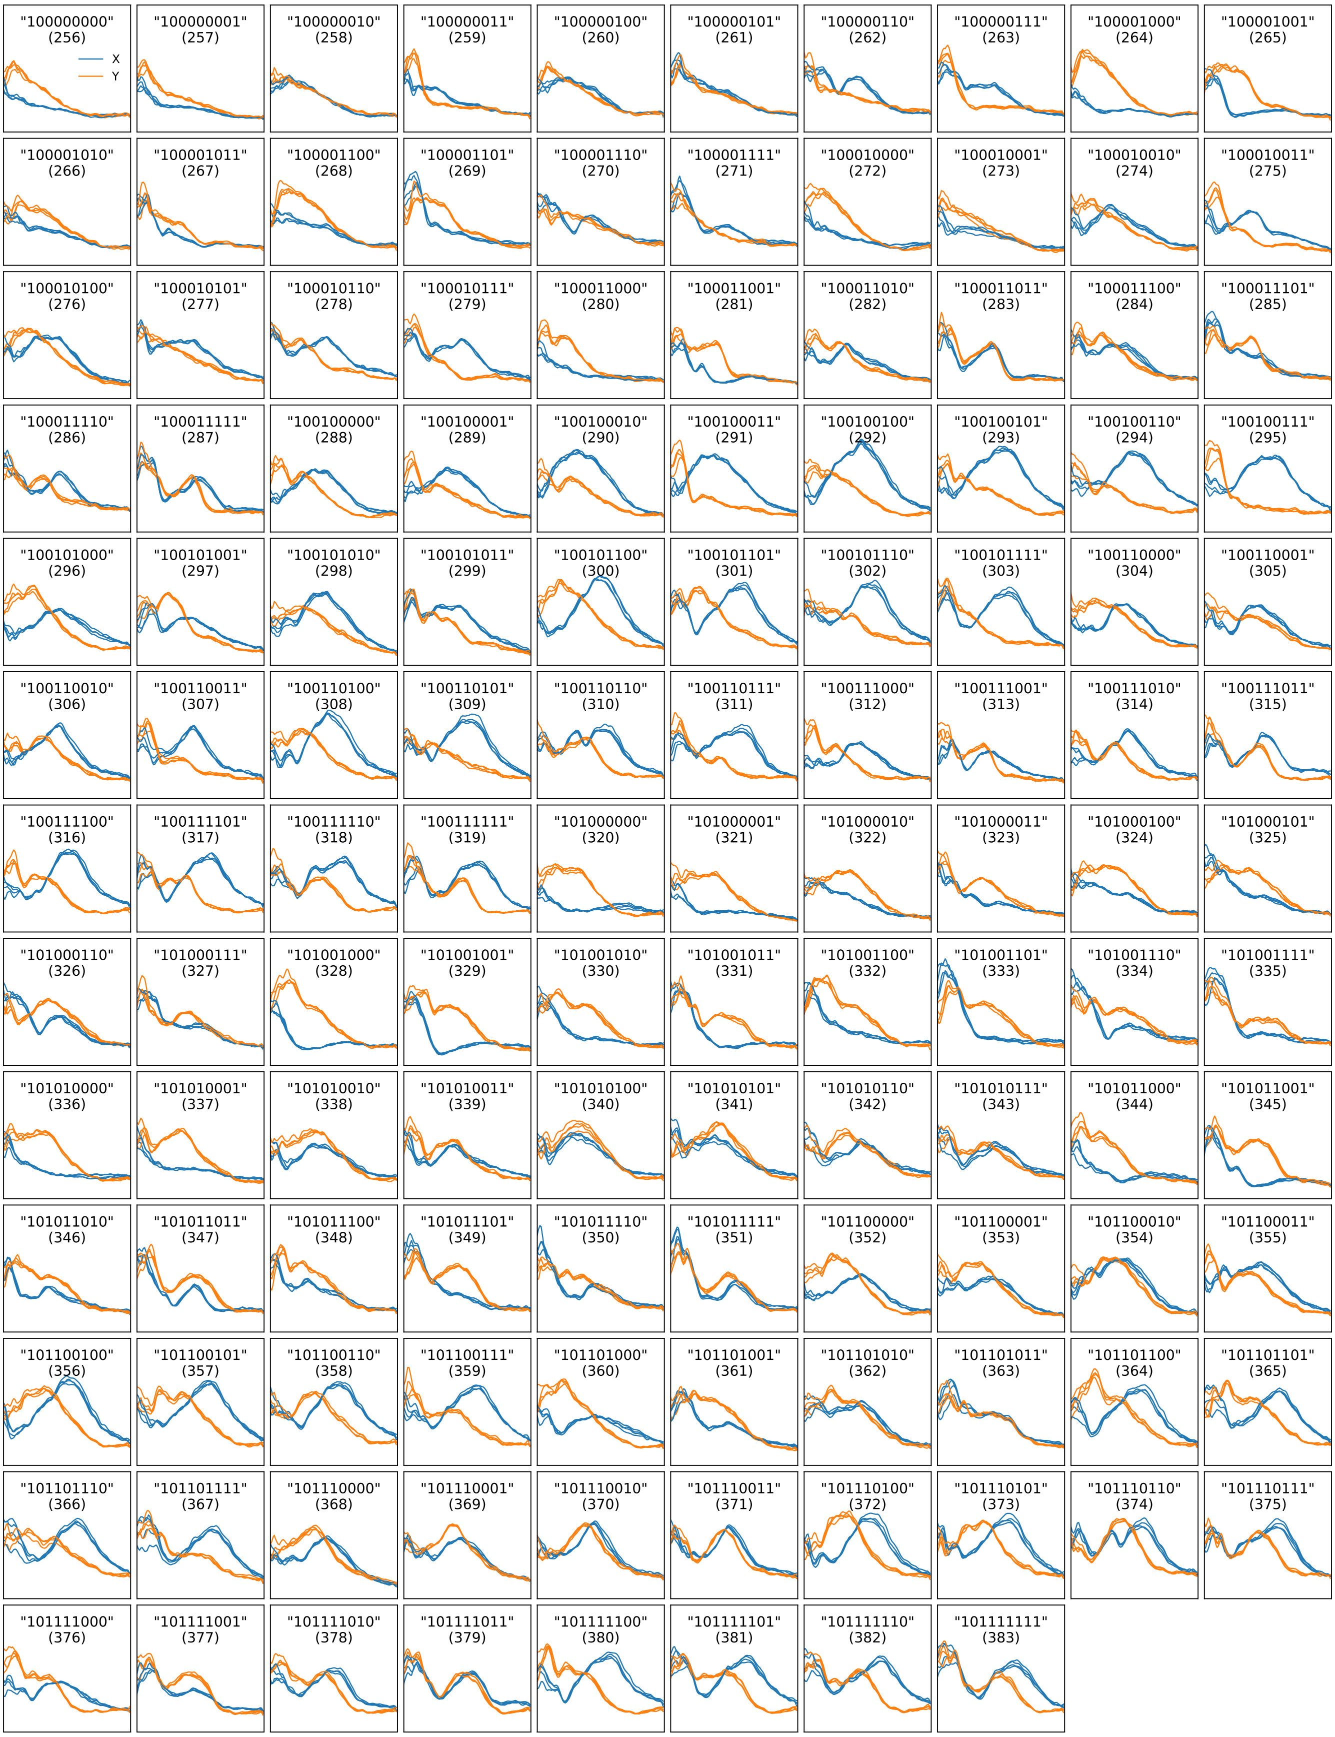


FIG. S.31. **Experimental spectra for the 9 bit structures 3/4** Structures 255-383.

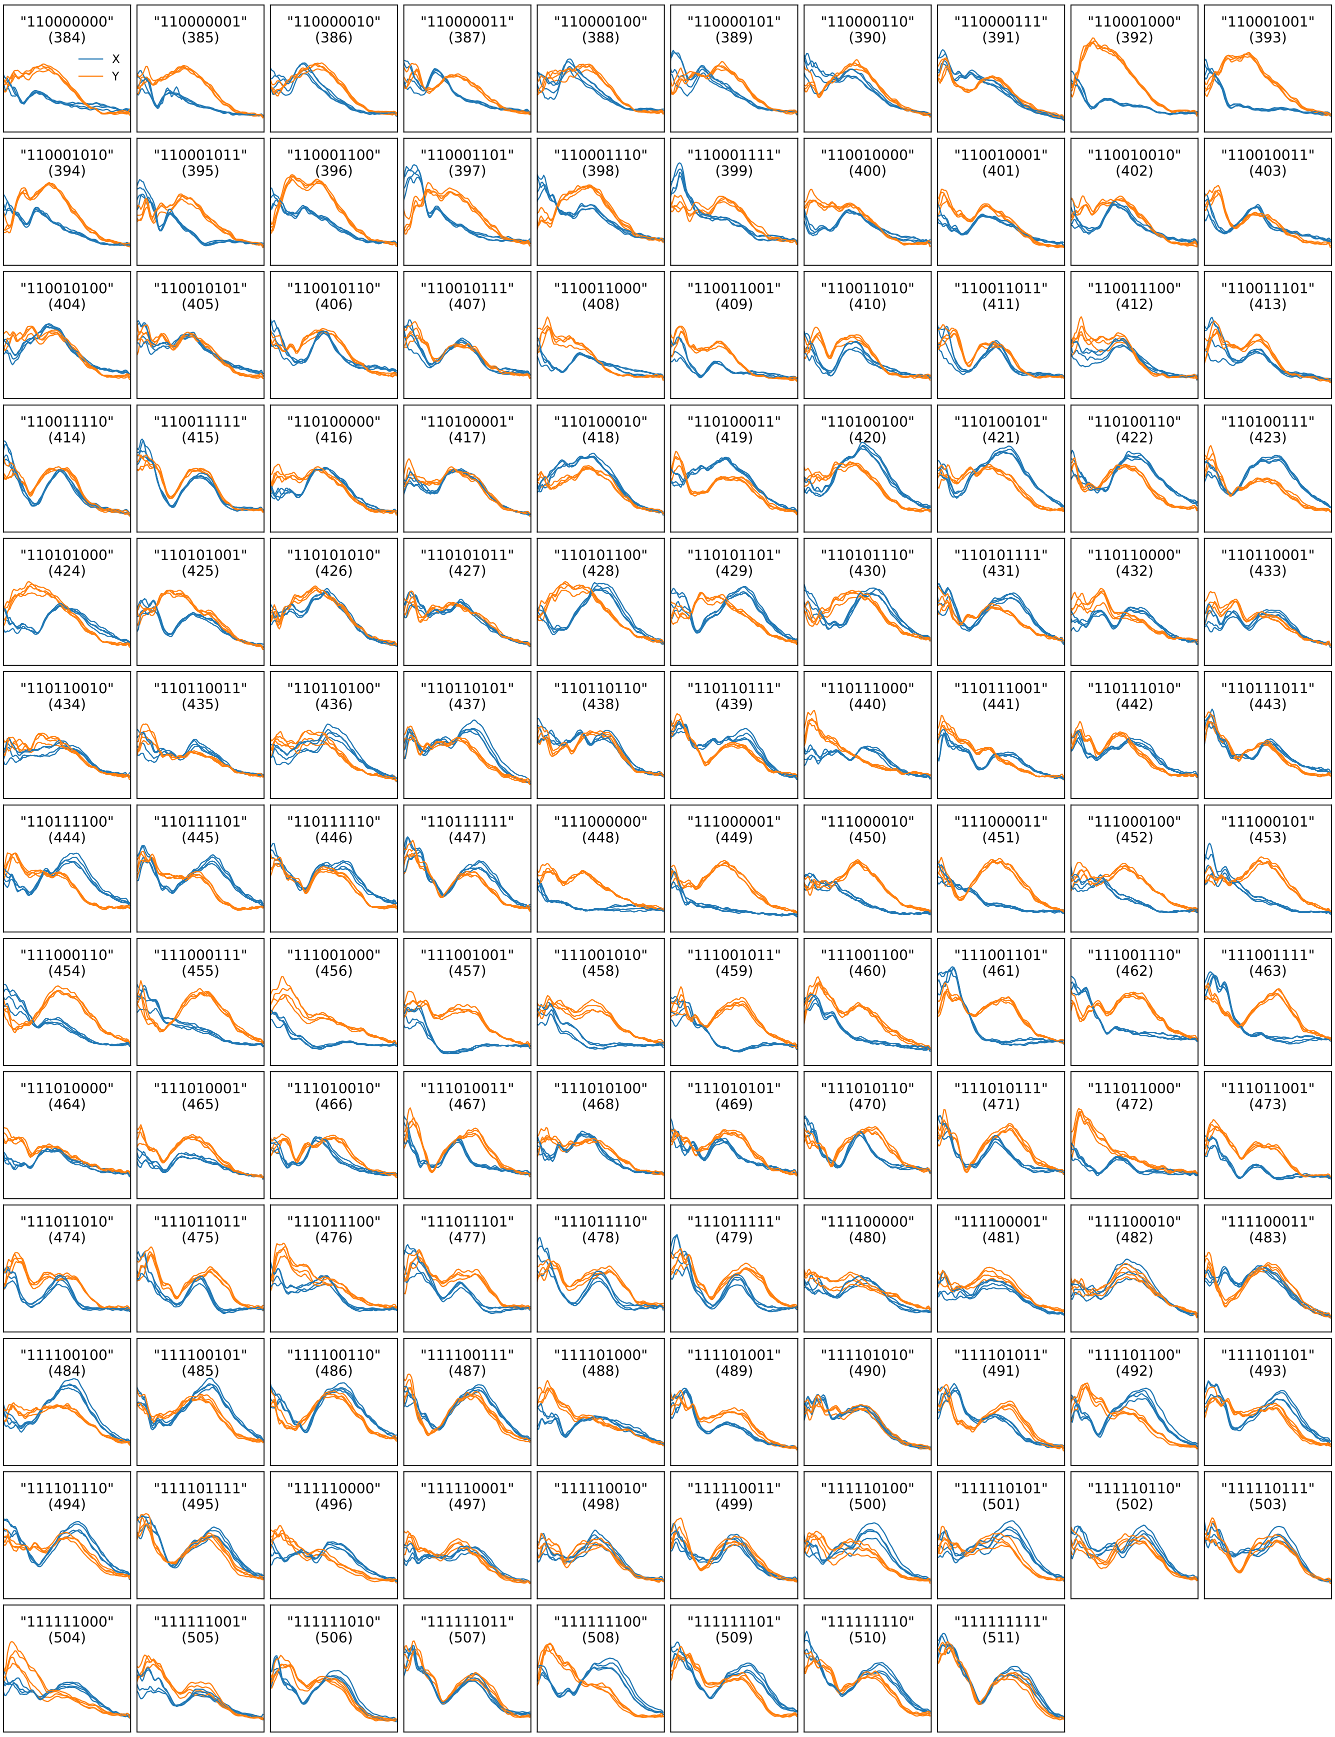


FIG. S.32. **Experimental spectra for the 9 bit structures 4/4** Structures 383-511.

## IX. FULLY NUMERICAL 9 BIT TRAINING SET

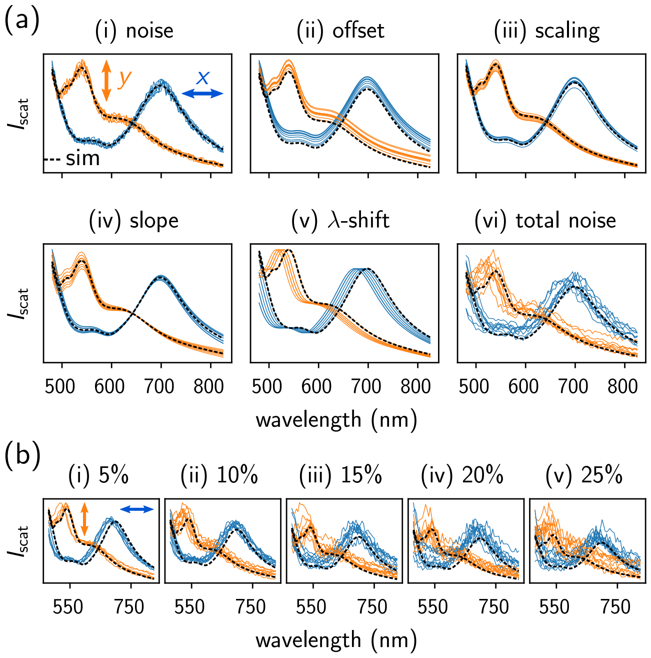


FIG. S.33. **Noise generation steps for fully numerical 9 bit dataset** (a) We numerically add noise to GDM simulated spectra of each structure via a sequence of random modifications, as illustrated here at the example of structure “001011010” (90). First we add random noise (i), and apply a random positive offset (ii) as well as a scaling factor (iii). Then we multiply the spectra with a linear function of random slope (iv) and finally apply a wavelength-shift (v). In order to do so, in the first place we simulated the spectra on an extended wavelength range. (b) several of such randomly modified spectra for different noise magnitudes between 5% (i) and 25% (v).

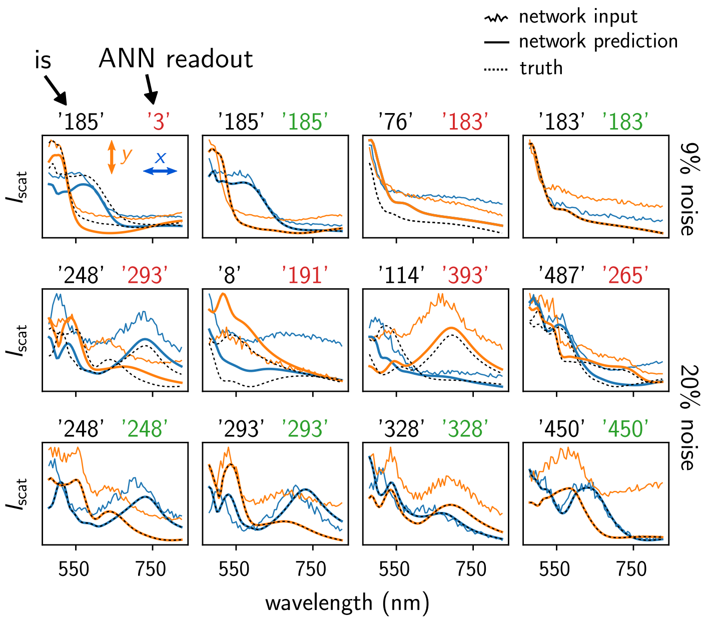


FIG. S.34. **Selected 9-bit structure spectra and the according network classification results** Selected read-out examples for 9% noise (top row) and 20% noise (middle and bottom rows). Green: correct, red: failed classification. The both incorrect 9% noise examples are the only two cases of failure in the whole validation set, composed of 10240 sample spectra.

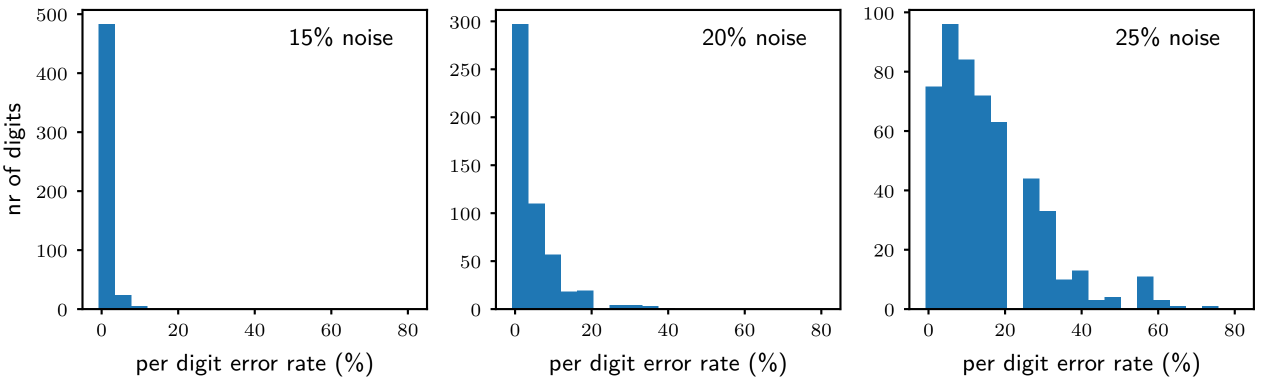


FIG. S.35. **Read-out error rates of the individual 9 bit pattern structures** Histograms of the error rates per individual binary 9-bit geometry for 15%, 20% and 25% noise level (from left to right). The 15% noise case leads only to a small number of errors, most of which with only 1 mistake out of 20 test-candidates per geometry (= 5% error). The datasets with 20% and 25% noise magnitude have significantly worse read-out accuracies for an increasing number of binary geometries.

## X. CONSIDERATIONS ON THE FEASIBLE INFORMATION DENSITY – 9 BIT STRUCTURE

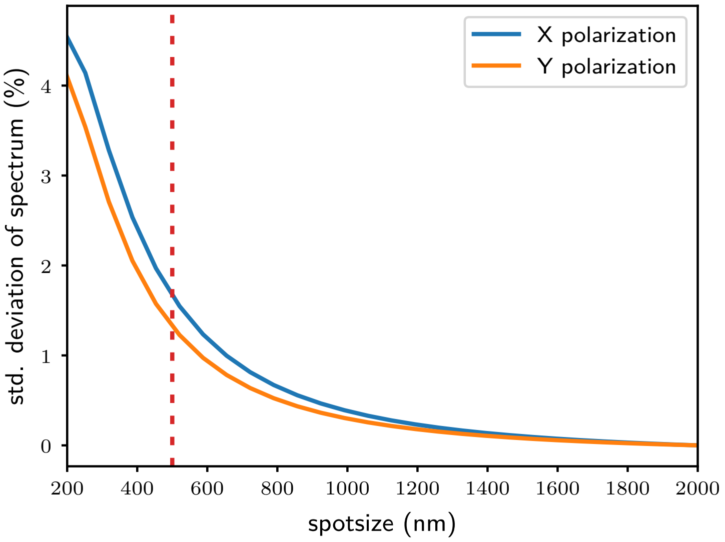


FIG. S.36. **Assessing the influence of a focused illumination on the scattering spectra** Standard deviation of the scattering intensity from a focused illuminated structure. Normalized to the spectrum obtained with plane wave illumination (at the example of the 9 bit structure "001010000"; considered spectral range 450 nm $\leq \lambda \leq$ 850 nm). "0%" means that besides a global scaling factor, the spectral response is identical to the plane wave case. The vertical, dashed line corresponds to a focal spot with a Gaussian waist of $w = 500$ nm, as used in figure S.37.

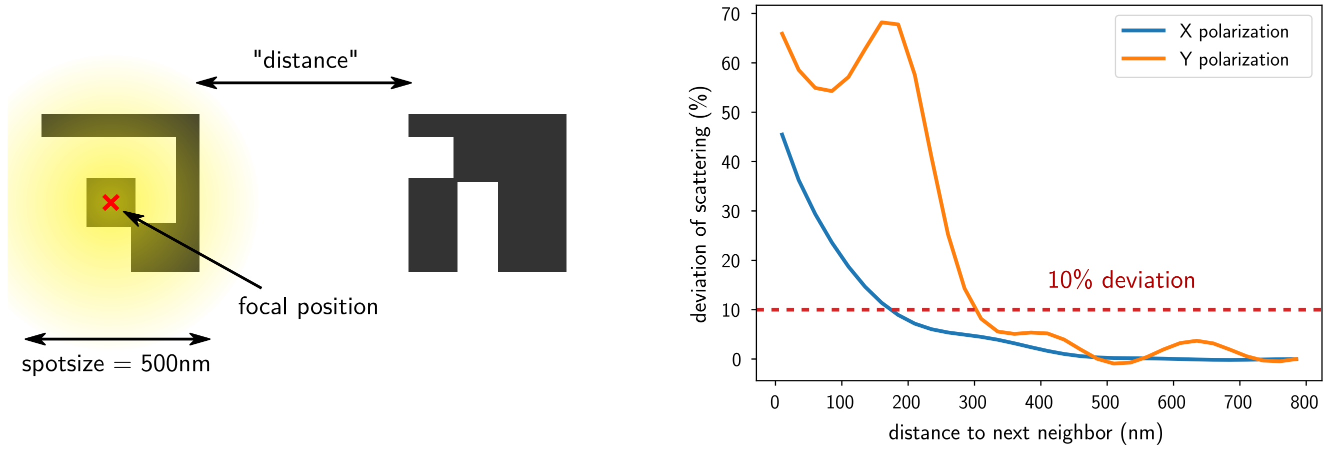


FIG. S.37. **Assessing the influence of nearby neighbor structures on the scattering spectra** Left: Illustration of the problem. A 9 bit structure (top view; on the left, "001010000") is illuminated by a narrowly focused white light source (a red cross indicates the focal position, the Gaussian waist of the spot is $w = 500$ nm). A second 9 bit nanostructure (here: "101101011") is positioned at a certain distance to the illuminated structure. The scattering from the total system is evaluated at $\lambda = 650$ nm for $X$ and $Y$ polarization as a function of the distance between the two structures (right plot). A red dashed line indicates the limit of 10% deviation with respect to the spectrum of the isolated structure. 10% deviation are assumed to be the limit for an error-free readout (see main text). Within this constraint, the two structures can be put together as close as $\approx$ 300 nm.
